# Supplementary material for: Minimally subtracted six loop renormalization of $O(n)$-symmetric $\phi^4$ theory and critical exponents
Source: arXiv:1705.06483 ancillary file (2017-09-24)

# Resummation of 6-loop $\varepsilon$ -expansions of $O(n)$ critical exponents

Mikhail V. Kompaniets

Erik Panzer

## 1 Introduction

This document contains details about the resummation of the critical exponents  $f \in \{\eta, \nu^{-1}, \omega\}$  as described in the article: We compute resummations and error estimates

$$E_\ell^f(\theta) := \delta_\ell + \text{Var}_b^{\ell-1, \ell} + \text{Var}_\lambda \left( \tilde{f}_\ell^\theta \right) + \text{Var}_q \left( \tilde{f}_\ell^\theta \right). \quad (1)$$

over a range of the parameters  $\theta = (b, \lambda, q)$ , where we use the abbreviations

$$\delta_\ell := \max \left\{ \left| \tilde{f}_\ell^\theta - \tilde{f}_{\ell-1}^\theta \right|, \left| \tilde{f}_\ell^\theta - \tilde{f}_{\ell-2}^\theta \right| \right\} \quad \text{and} \quad (2)$$

$$\text{Var}_b^{\ell-1, \ell} := \max \left\{ \text{Var}_b \left( \tilde{f}_\ell^\theta \right), \text{Var}_b \left( \tilde{f}_{\ell-1}^\theta \right) \right\}. \quad (3)$$

For each resummation (indexed by  $f$ , the dimension, the internal degrees  $n$  of freedom, and the loop order  $\ell$ ), we show the point  $(b, \lambda, q)$  with the smallest error estimate, denoted by  $\bar{E}$ , and provide plots illustrating the sensitivity of the this resummation with respect to variations of the parameters  $b$  and  $\lambda$ , one at a time. The various curves show the resummations for different perturbative orders:

$$\varepsilon^{\leq 3}: \quad \text{.....} \quad \varepsilon^{\leq 4}: \quad \text{---} \quad \varepsilon^{\leq 5}: \quad \text{---} \quad \varepsilon^{\leq 6}: \quad \text{---}$$

Furthermore, we include plots of the points  $(\tilde{f}_\ell^\theta, E_\ell^f(\theta))$  for all resummations  $\theta = (b, \lambda, q)$  with error estimates at most  $3\bar{E}$ . These provide an indication of how well the error estimates capture the actual spread of resummations. Also they reveal whether the minimum  $\bar{E}$  of  $E$  (the “apparently best” resummation, illustrated in the other plots) is sharp—or if several different resummations yield similarly small error estimates. We report the standard deviation  $\sigma$  of these resummations, which we add twice to  $\bar{E}_\ell^f$  to obtain the errors reported for the critical exponents in sections 6 and 7 of the paper. In the plot, the “apparently best” resummation lies on the lower horizontal axis and is marked in red. For most cases, these are the values for the critical exponents reported in sections 6 and 7 of the paper.

However, as discussed in the paper, in a few cases several different resummations share a very small error estimate. It can then happen that the “apparently best” resummation appears to be biased, and a more faithful representation of the data seems to be given by a kind of average. We therefore also show the weighted average

$$\sum_{\theta: E_\ell^f(\theta) < 3\bar{E}_\ell^f} \tilde{f}_\ell^\theta / [E_\ell^f(\theta)]^2 \bigg/ \sum_{\theta: E_\ell^f(\theta) < 3\bar{E}_\ell^f} 1 / [E_\ell^f(\theta)]^2 \quad (4)$$

in the plots, as a vertical dashed line.

## $D = 3$ dimensions

### $\eta(n=0)$ : 5 loops

Minimal error:  $\overline{E} = \overline{E}_5^\eta = 0.00047$  for  $\hat{\eta}_5^{b,\lambda,q} = 0.03139$  at  $b = 7.5$ ,  $\lambda = 2.52$ ,  $q = 0.24$

$$\delta_5 = 0.00003, \quad \text{Var}_b^{4,5} = 0.00024, \quad \text{Var}_\lambda = 0.00006, \quad \text{Var}_q = 0.00015$$

Weighted mean of  $\hat{\eta}_5^\theta$  with  $E_5^\eta(\theta) < 3\overline{E}$ : 0.03150, standard deviation:  $\sigma = 0.00030$

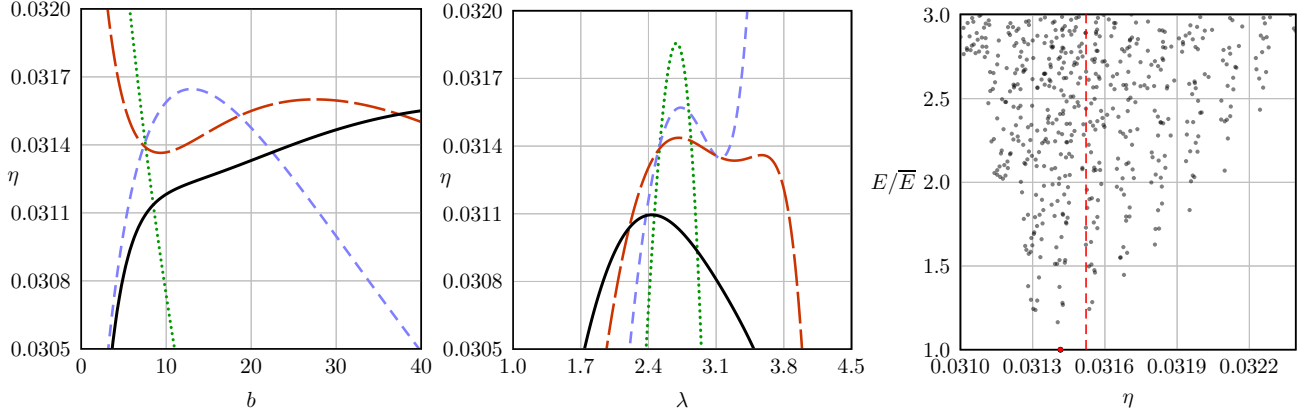

### $\eta(n=0)$ : 6 loops

Minimal error:  $\overline{E} = \overline{E}_6^\eta = 0.00021$  for  $\hat{\eta}_6^{b,\lambda,q} = 0.03100$  at  $b = 11.0$ ,  $\lambda = 2.54$ ,  $q = 0.20$

$$\delta_6 = 0.00001, \quad \text{Var}_b^{5,6} = 0.00004, \quad \text{Var}_\lambda = 0.00005, \quad \text{Var}_q = 0.00011$$

Weighted mean of  $\hat{\eta}_6^\theta$  with  $E_6^\eta(\theta) < 3\overline{E}$ : 0.03083, standard deviation:  $\sigma = 0.00023$

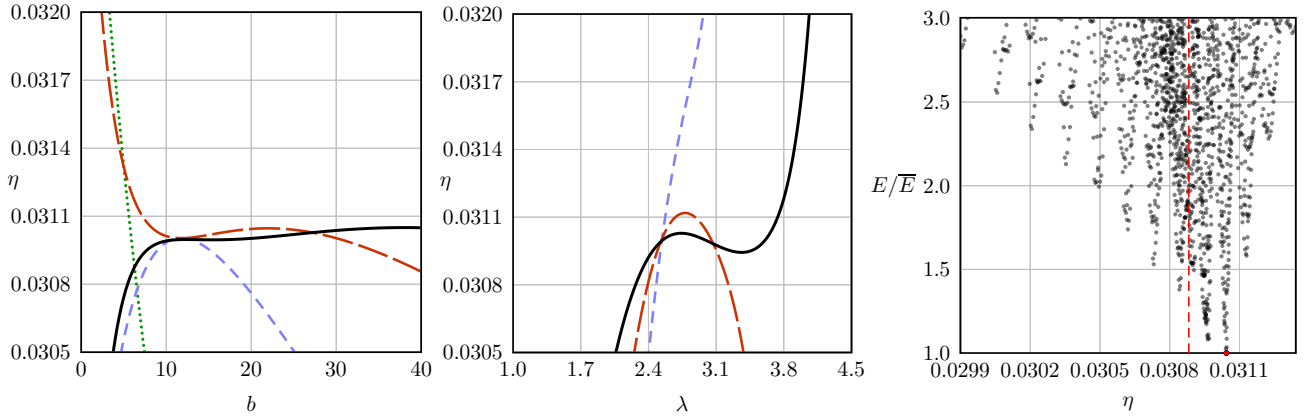

$\eta(n=1)$ : **5 loops**

Minimal error:  $\overline{E} = \overline{E}_5^\eta = 0.00050$  for  $\hat{\eta}_5^{b,\lambda,q} = 0.03655$  at  $b = 8.0$ ,  $\lambda = 2.50$ ,  $q = 0.24$

$$\delta_5 = 0.00003, \quad \text{Var}_b^{4,5} = 0.00024, \quad \text{Var}_\lambda = 0.00006, \quad \text{Var}_q = 0.00017$$

Weighted mean of  $\hat{\eta}_5^\theta$  with  $E_5^\eta(\theta) < 3\overline{E}$ : 0.03669, standard deviation:  $\sigma = 0.00031$

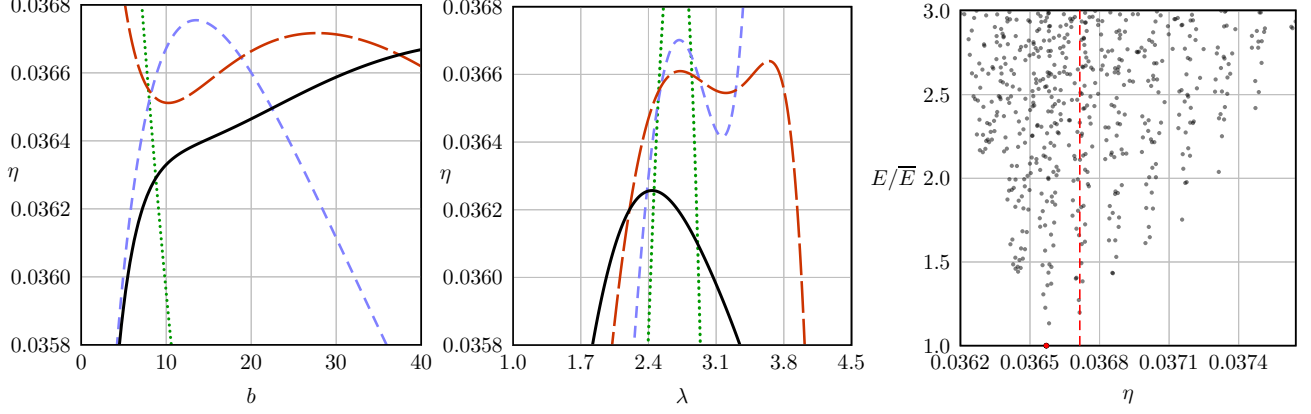

$\eta(n=1)$ : **6 loops**

Minimal error:  $\overline{E} = \overline{E}_6^\eta = 0.00020$  for  $\hat{\eta}_6^{b,\lambda,q} = 0.03615$  at  $b = 11.0$ ,  $\lambda = 2.56$ ,  $q = 0.20$

$$\delta_6 = 0.00000, \quad \text{Var}_b^{5,6} = 0.00006, \quad \text{Var}_\lambda = 0.00003, \quad \text{Var}_q = 0.00011$$

Weighted mean of  $\hat{\eta}_6^\theta$  with  $E_6^\eta(\theta) < 3\overline{E}$ : 0.03603, standard deviation:  $\sigma = 0.00020$

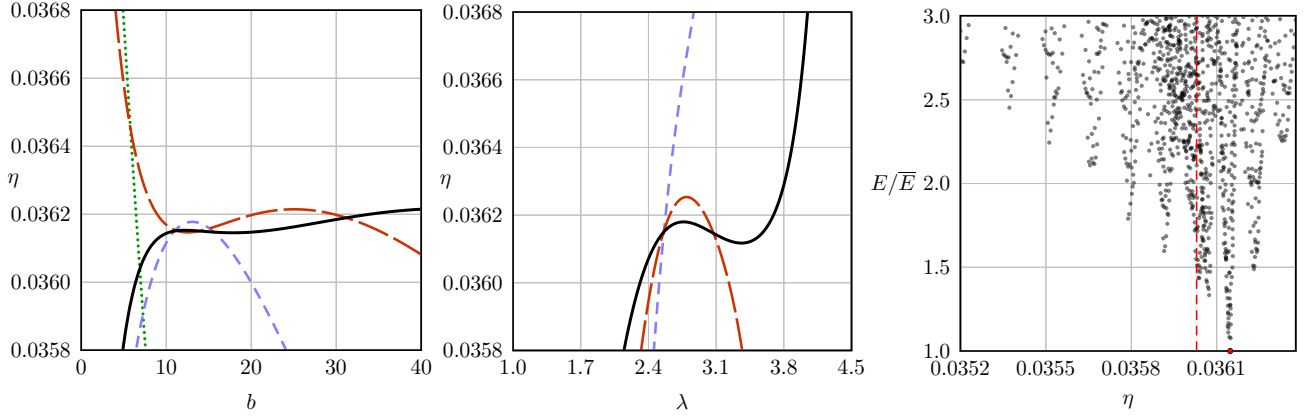

$\eta(n=2)$ : **5 loops**

Minimal error:  $\overline{E} = \overline{E}_5^\eta = 0.00046$  for  $\hat{\eta}_5^{b,\lambda,q} = 0.03837$  at  $b = 8.5$ ,  $\lambda = 2.46$ ,  $q = 0.24$

$$\delta_5 = 0.00002, \quad \text{Var}_b^{4,5} = 0.00021, \quad \text{Var}_\lambda = 0.00006, \quad \text{Var}_q = 0.00017$$

Weighted mean of  $\hat{\eta}_5^\theta$  with  $E_5^\eta(\theta) < 3\overline{E}$ : 0.03846, standard deviation:  $\sigma = 0.00029$

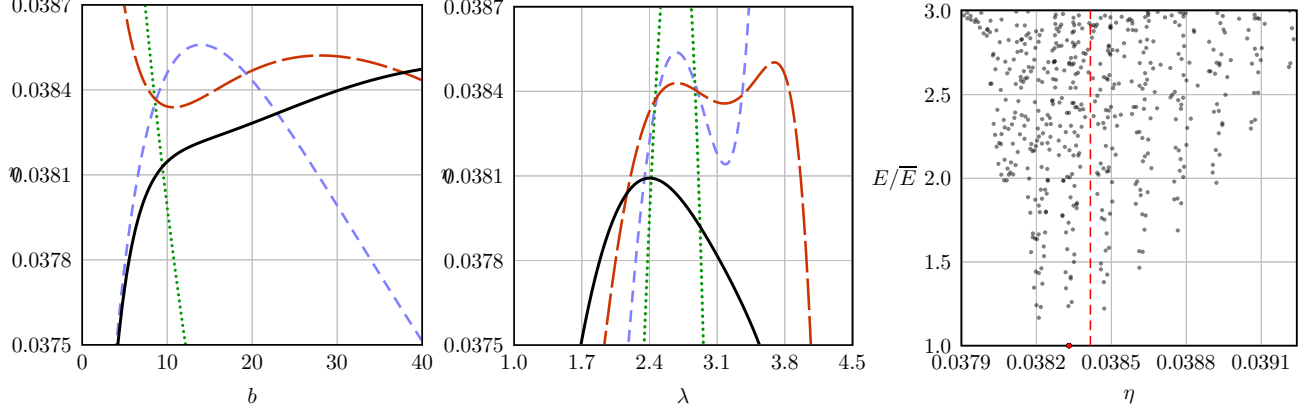

$\eta(n=2)$ : **6 loops**

Minimal error:  $\overline{E} = \overline{E}_6^\eta = 0.00020$  for  $\hat{\eta}_6^{b,\lambda,q} = 0.03798$  at  $b = 11.5$ ,  $\lambda = 2.52$ ,  $q = 0.20$

$$\delta_6 = 0.00004, \quad \text{Var}_b^{5,6} = 0.00003, \quad \text{Var}_\lambda = 0.00003, \quad \text{Var}_q = 0.00010$$

Weighted mean of  $\hat{\eta}_6^\theta$  with  $E_6^\eta(\theta) < 3\overline{E}$ : 0.03787, standard deviation:  $\sigma = 0.00019$

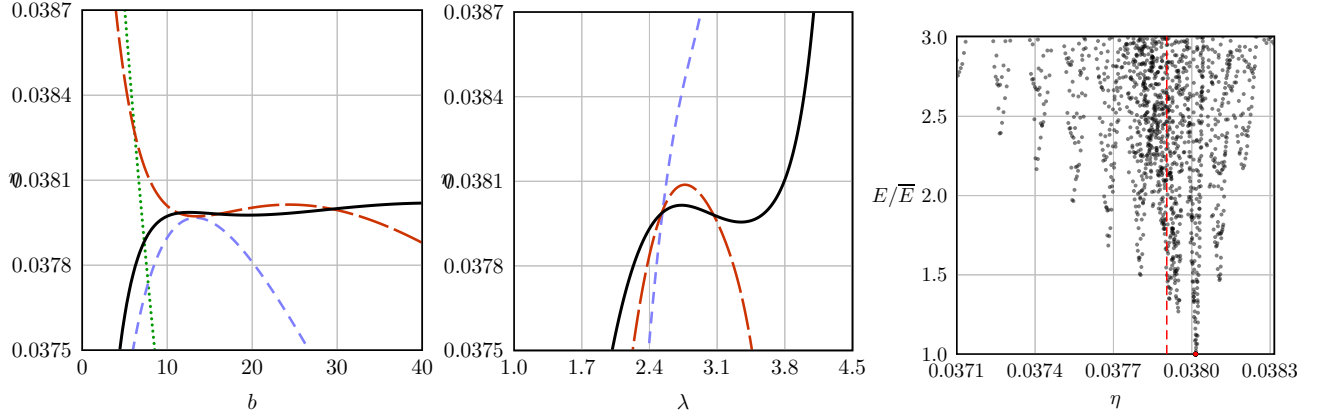

$\eta(n=3)$ : **5 loops**

Minimal error:  $\overline{E} = \overline{E}_5^\eta = 0.00045$  for  $\hat{\eta}_5^{b,\lambda,q} = 0.03817$  at  $b = 9.0$ ,  $\lambda = 2.46$ ,  $q = 0.22$

$$\delta_5 = 0.00004, \quad \text{Var}_b^{4,5} = 0.00019, \quad \text{Var}_\lambda = 0.00006, \quad \text{Var}_q = 0.00015$$

Weighted mean of  $\hat{\eta}_5^\theta$  with  $E_5^\eta(\theta) < 3\overline{E}$ : 0.03828, standard deviation:  $\sigma = 0.00027$

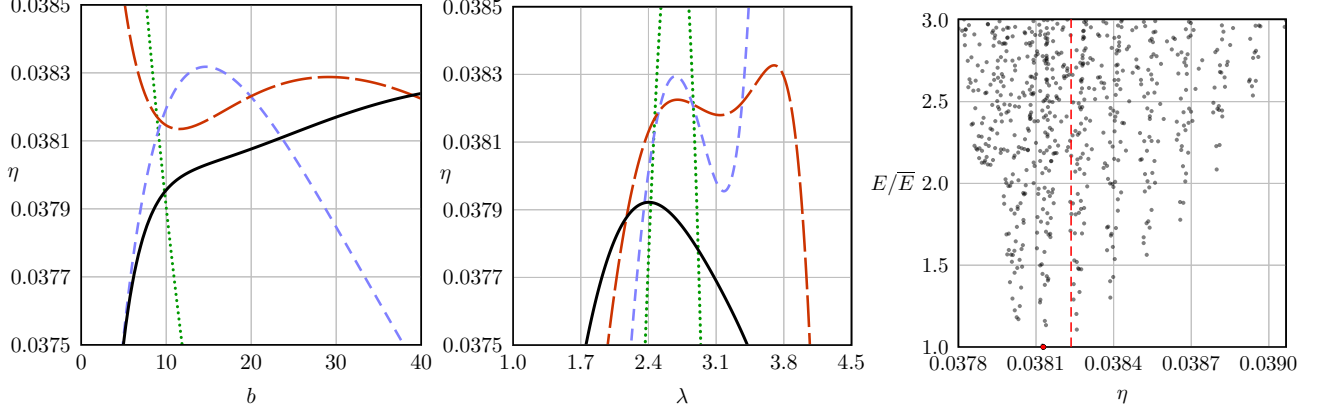

$\eta(n=3)$ : **6 loops**

Minimal error:  $\overline{E} = \overline{E}_6^\eta = 0.00018$  for  $\hat{\eta}_6^{b,\lambda,q} = 0.03783$  at  $b = 12.0$ ,  $\lambda = 2.56$ ,  $q = 0.18$

$$\delta_6 = 0.00000, \quad \text{Var}_b^{5,6} = 0.00007, \quad \text{Var}_\lambda = 0.00002, \quad \text{Var}_q = 0.00009$$

Weighted mean of  $\hat{\eta}_6^\theta$  with  $E_6^\eta(\theta) < 3\overline{E}$ : 0.03775, standard deviation:  $\sigma = 0.00017$

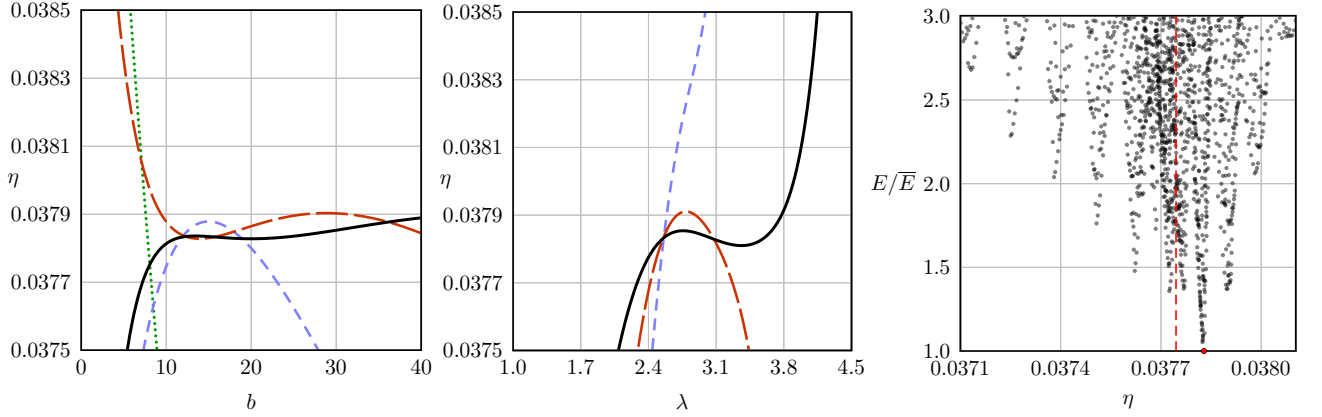

$\eta(n=4)$ : **5 loops**

Minimal error:  $\overline{E} = \overline{E}_5^\eta = 0.00041$  for  $\hat{\eta}_5^{b,\lambda,q} = 0.03696$  at  $b = 9.5$ ,  $\lambda = 2.44$ ,  $q = 0.20$

$$\delta_5 = 0.00005, \quad \text{Var}_b^{4,5} = 0.00017, \quad \text{Var}_\lambda = 0.00005, \quad \text{Var}_q = 0.00014$$

Weighted mean of  $\hat{\eta}_5^\theta$  with  $E_5^\eta(\theta) < 3\overline{E}$ : 0.03704, standard deviation:  $\sigma = 0.00024$

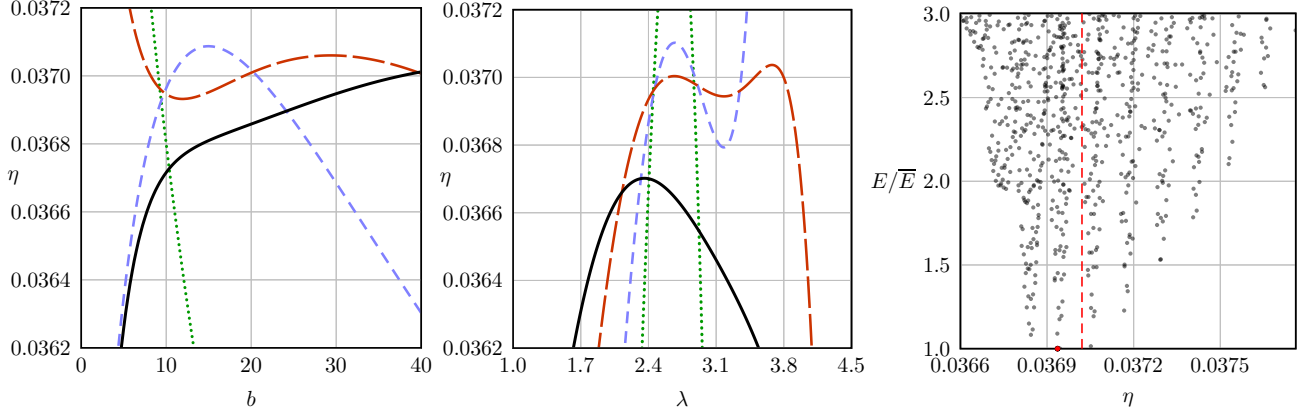

$\eta(n=4)$ : **6 loops**

Minimal error:  $\overline{E} = \overline{E}_6^\eta = 0.00016$  for  $\hat{\eta}_6^{b,\lambda,q} = 0.03663$  at  $b = 14.0$ ,  $\lambda = 2.52$ ,  $q = 0.16$

$$\delta_6 = 0.00001, \quad \text{Var}_b^{5,6} = 0.00003, \quad \text{Var}_\lambda = 0.00004, \quad \text{Var}_q = 0.00009$$

Weighted mean of  $\hat{\eta}_6^\theta$  with  $E_6^\eta(\theta) < 3\overline{E}$ : 0.03653, standard deviation:  $\sigma = 0.00014$

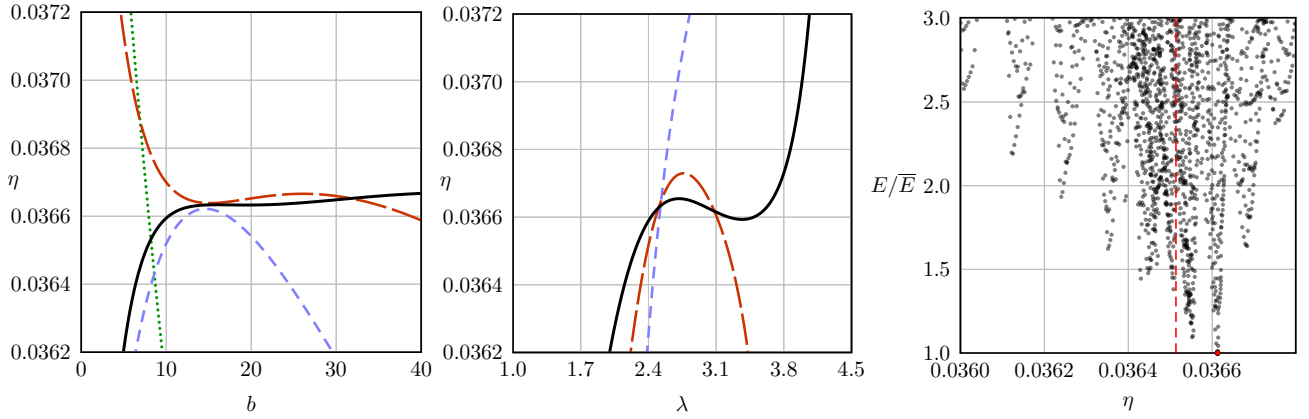

$\nu^{-1}(n=0)$ : **5 loops**

Minimal error:  $\overline{E} = \overline{E}_5^{\nu^{-1}} = 0.00164$  for  $\widetilde{\nu^{-1}}_5^{b,\lambda,q} = 1.70272$  at  $b = 9.5$ ,  $\lambda = 1.48$ ,  $q = 0.02$

$$\delta_5 = 0.00027, \quad \text{Var}_b^{4,5} = 0.00067, \quad \text{Var}_\lambda = 0.00053, \quad \text{Var}_q = 0.00017$$

Weighted mean of  $\widetilde{\nu^{-1}}_5^\theta$  with  $E_5^{\nu^{-1}}(\theta) < 3\overline{E}$ : 1.70124, standard deviation:  $\sigma = 0.00111$

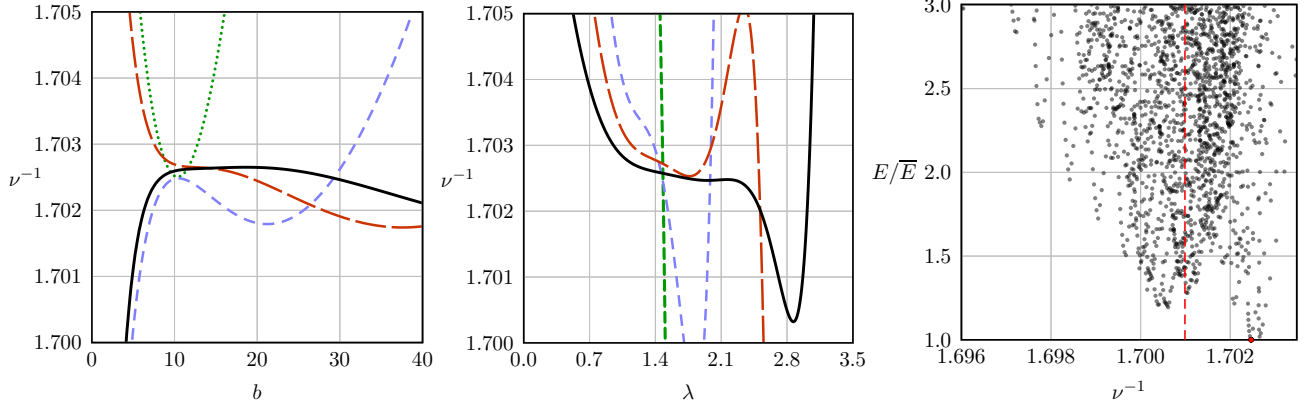

$\nu^{-1}(n=0)$ : **6 loops**

Minimal error:  $\overline{E} = \overline{E}_6^{\nu^{-1}} = 0.00041$  for  $\widetilde{\nu^{-1}}_6^{b,\lambda,q} = 1.70251$  at  $b = 10.0$ ,  $\lambda = 1.42$ ,  $q = 0.04$

$$\delta_6 = 0.00005, \quad \text{Var}_b^{5,6} = 0.00021, \quad \text{Var}_\lambda = 0.00006, \quad \text{Var}_q = 0.00009$$

Weighted mean of  $\widetilde{\nu^{-1}}_6^\theta$  with  $E_6^{\nu^{-1}}(\theta) < 3\overline{E}$ : 1.70246, standard deviation:  $\sigma = 0.00016$

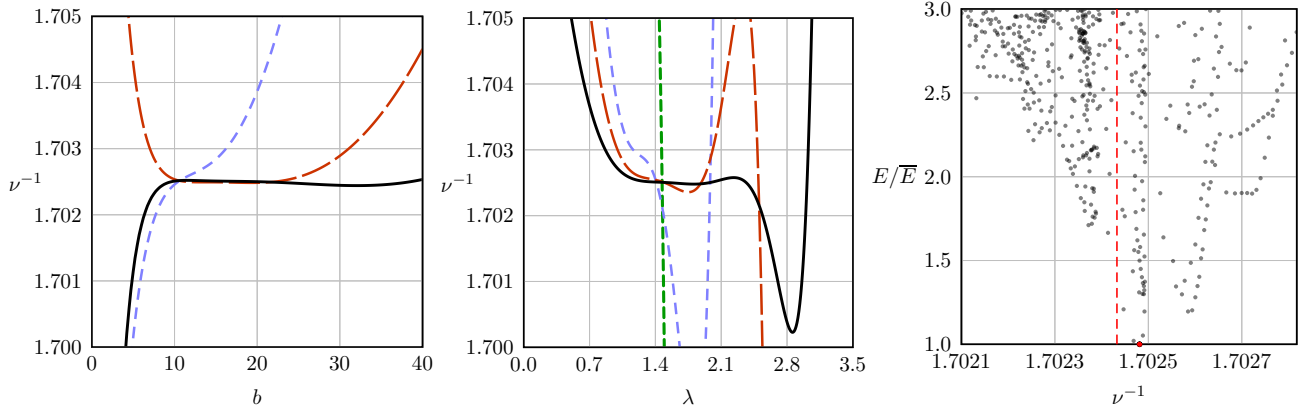

$\nu^{-1}(n=1)$ : **5 loops**

Minimal error:  $\overline{E} = \overline{E}_5^{\nu^{-1}} = 0.00196$  for  $\widetilde{\nu^{-1}}_5^{b,\lambda,q} = 1.58992$  at  $b = 10.0$ ,  $\lambda = 1.46$ ,  $q = 0.12$

$$\delta_5 = 0.00064, \quad \text{Var}_b^{4,5} = 0.00063, \quad \text{Var}_\lambda = 0.00046, \quad \text{Var}_q = 0.00023$$

Weighted mean of  $\widetilde{\nu^{-1}}_5^\theta$  with  $E_5^{\nu^{-1}}(\theta) < 3\overline{E}$ : 1.58878, standard deviation:  $\sigma = 0.00156$

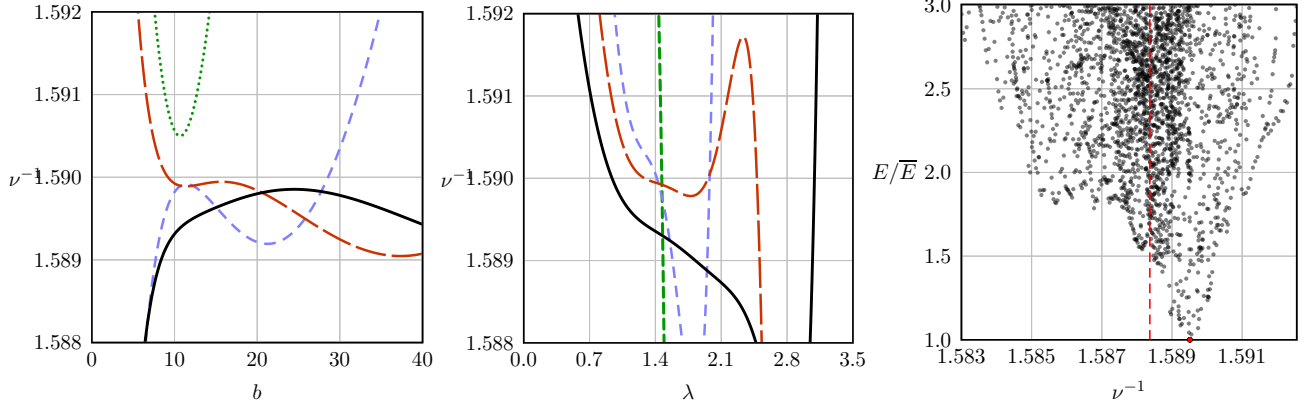

$\nu^{-1}(n=1)$ : **6 loops**

Minimal error:  $\overline{E} = \overline{E}_6^{\nu^{-1}} = 0.00061$  for  $\widetilde{\nu^{-1}}_6^{b,\lambda,q} = 1.58919$  at  $b = 13.0$ ,  $\lambda = 1.30$ ,  $q = 0.16$

$$\delta_6 = 0.00014, \quad \text{Var}_b^{5,6} = 0.00022, \quad \text{Var}_\lambda = 0.00005, \quad \text{Var}_q = 0.00019$$

Weighted mean of  $\widetilde{\nu^{-1}}_6^\theta$  with  $E_6^{\nu^{-1}}(\theta) < 3\overline{E}$ : 1.58924, standard deviation:  $\sigma = 0.00026$

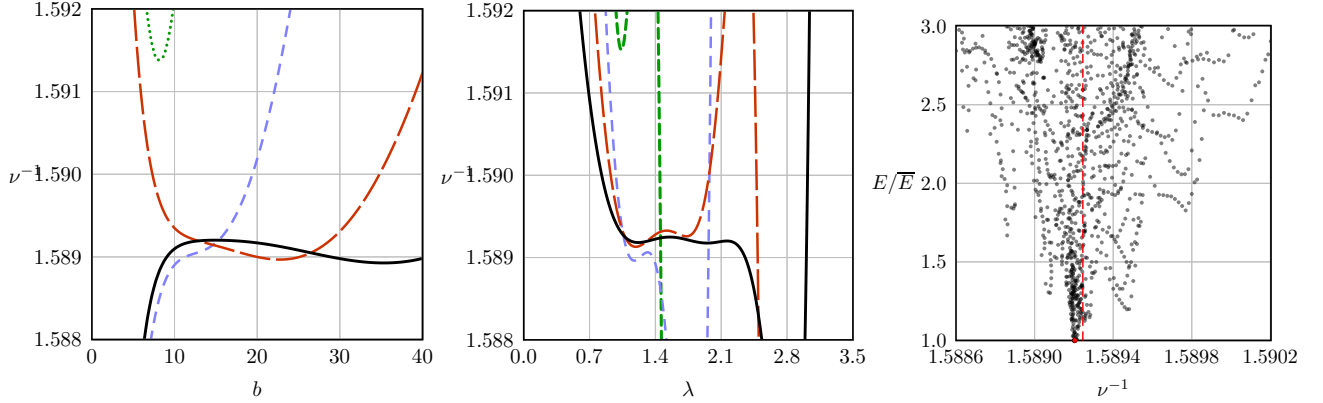



$\nu^{-1}(n=2)$ : **5 loops**

Minimal error:  $\overline{E} = \overline{E}_5^{\nu^{-1}} = 0.00156$  for  $\widetilde{\nu^{-1}}_5^{b,\lambda,q} = 1.49534$  at  $b = 10.5$ ,  $\lambda = 1.04$ ,  $q = 0.24$

$$\delta_5 = 0.00007, \quad \text{Var}_b^{4,5} = 0.00075, \quad \text{Var}_\lambda = 0.00015, \quad \text{Var}_q = 0.00057$$

Weighted mean of  $\widetilde{\nu^{-1}}_5^\theta$  with  $E_5^{\nu^{-1}}(\theta) < 3\overline{E}$ : 1.49512, standard deviation:  $\sigma = 0.00072$

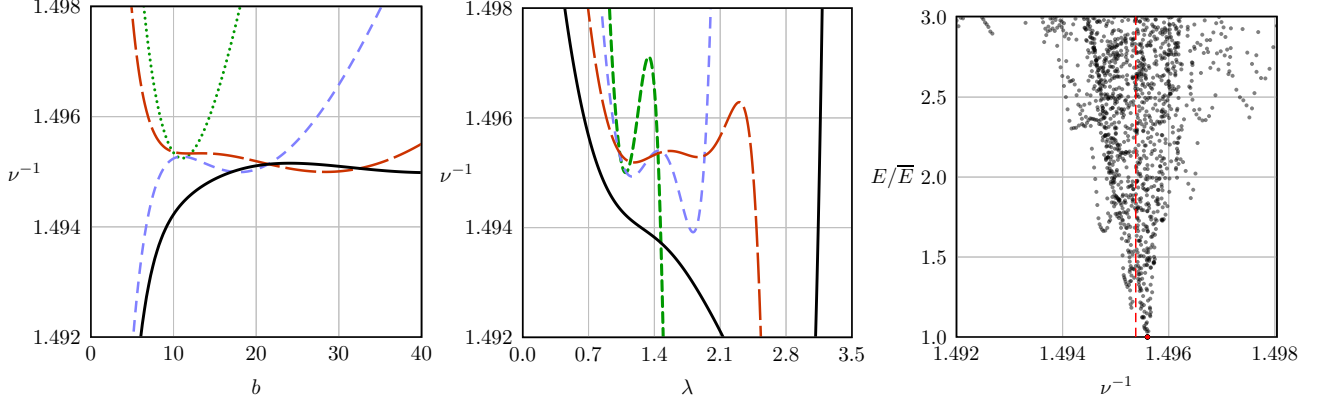

$\nu^{-1}(n=2)$ : **6 loops**

Minimal error:  $\overline{E} = \overline{E}_6^{\nu^{-1}} = 0.00098$  for  $\widetilde{\nu^{-1}}_6^{b,\lambda,q} = 1.49490$  at  $b = 20.5$ ,  $\lambda = 1.22$ ,  $q = 0.24$

$$\delta_6 = 0.00001, \quad \text{Var}_b^{5,6} = 0.00032, \quad \text{Var}_\lambda = 0.00017, \quad \text{Var}_q = 0.00048$$

Weighted mean of  $\widetilde{\nu^{-1}}_6^\theta$  with  $E_6^{\nu^{-1}}(\theta) < 3\overline{E}$ : 1.49475, standard deviation:  $\sigma = 0.00064$

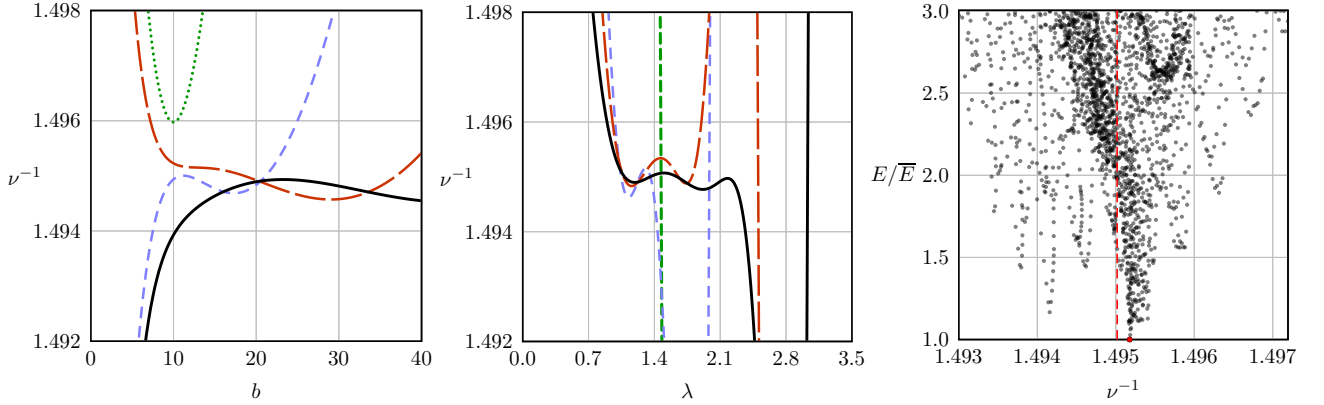

$\nu^{-1}(n=3)$ : **5 loops**

Minimal error:  $\overline{E} = \overline{E}_5^{\nu^{-1}} = 0.00171$  for  $\widetilde{\nu^{-1}}_5^{b,\lambda,q} = 1.41669$  at  $b = 9.5$ ,  $\lambda = 0.88$ ,  $q = 0.34$

$$\delta_5 = 0.00023, \quad \text{Var}_b^{4,5} = 0.00052, \quad \text{Var}_\lambda = 0.00033, \quad \text{Var}_q = 0.00063$$

Weighted mean of  $\widetilde{\nu^{-1}}_5^\theta$  with  $E_5^{\nu^{-1}}(\theta) < 3\overline{E}$ : 1.41732, standard deviation:  $\sigma = 0.00071$

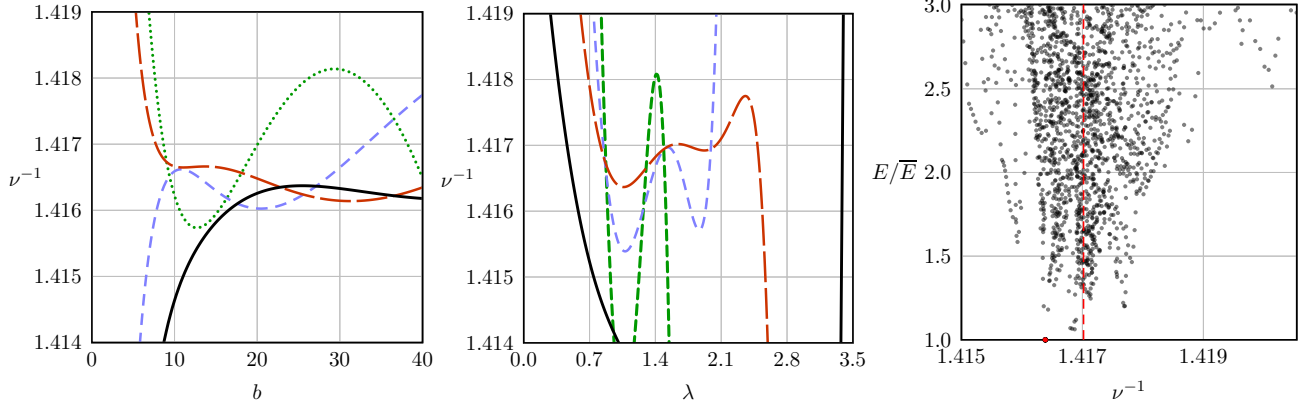

$\nu^{-1}(n=3)$ : **6 loops**

Minimal error:  $\overline{E} = \overline{E}_6^{\nu^{-1}} = 0.00149$  for  $\widetilde{\nu^{-1}}_6^{b,\lambda,q} = 1.41713$  at  $b = 25.5$ ,  $\lambda = 1.24$ ,  $q = 0.30$

$$\delta_6 = 0.00006, \quad \text{Var}_b^{5,6} = 0.00050, \quad \text{Var}_\lambda = 0.00031, \quad \text{Var}_q = 0.00063$$

Weighted mean of  $\widetilde{\nu^{-1}}_6^\theta$  with  $E_6^{\nu^{-1}}(\theta) < 3\overline{E}$ : 1.41661, standard deviation:  $\sigma = 0.00130$

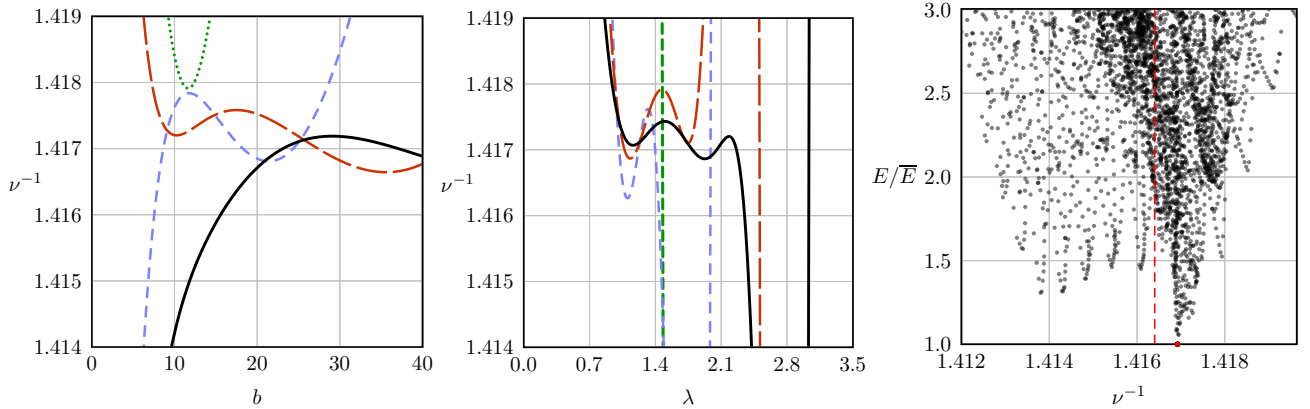

$\nu^{-1}(n=4)$ : **5 loops**

Minimal error:  $\overline{E} = \overline{E}_5^{\nu^{-1}} = 0.00202$  for  $\widetilde{\nu^{-1}}_5^{b,\lambda,q} = 1.35195$  at  $b = 10.0$ ,  $\lambda = 0.82$ ,  $q = 0.40$

$$\delta_5 = 0.00033, \quad \text{Var}_b^{4,5} = 0.00045, \quad \text{Var}_\lambda = 0.00052, \quad \text{Var}_q = 0.00072$$

Weighted mean of  $\widetilde{\nu^{-1}}_5^\theta$  with  $E_5^{\nu^{-1}}(\theta) < 3\overline{E}$ : 1.35336, standard deviation:  $\sigma = 0.00115$

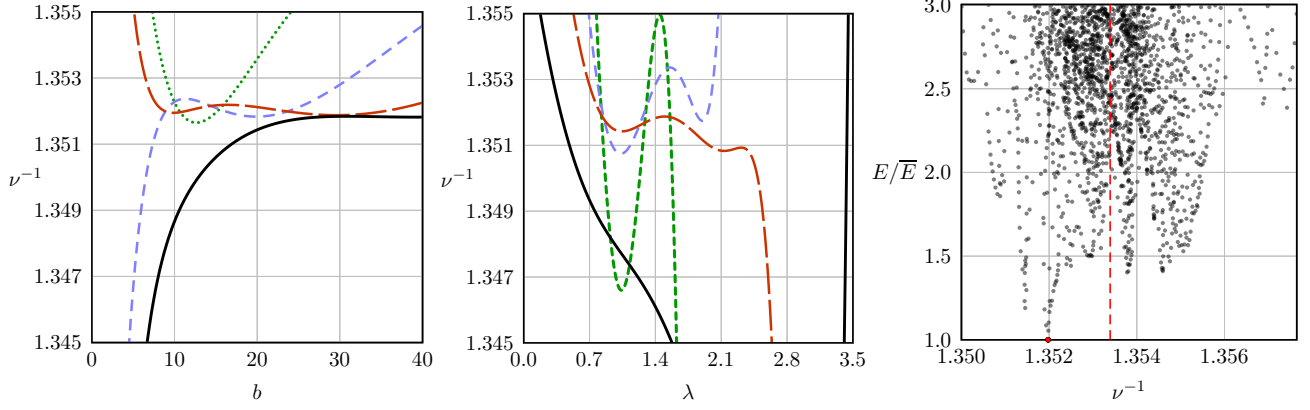

$\nu^{-1}(n=4)$ : **6 loops**

Minimal error:  $\overline{E} = \overline{E}_6^{\nu^{-1}} = 0.00221$  for  $\widetilde{\nu^{-1}}_6^{b,\lambda,q} = 1.34937$  at  $b = 17.0$ ,  $\lambda = 0.72$ ,  $q = 0.46$

$$\delta_6 = 0.00029, \quad \text{Var}_b^{5,6} = 0.00037, \quad \text{Var}_\lambda = 0.00076, \quad \text{Var}_q = 0.00080$$

Weighted mean of  $\widetilde{\nu^{-1}}_6^\theta$  with  $E_6^{\nu^{-1}}(\theta) < 3\overline{E}$ : 1.35196, standard deviation:  $\sigma = 0.00207$

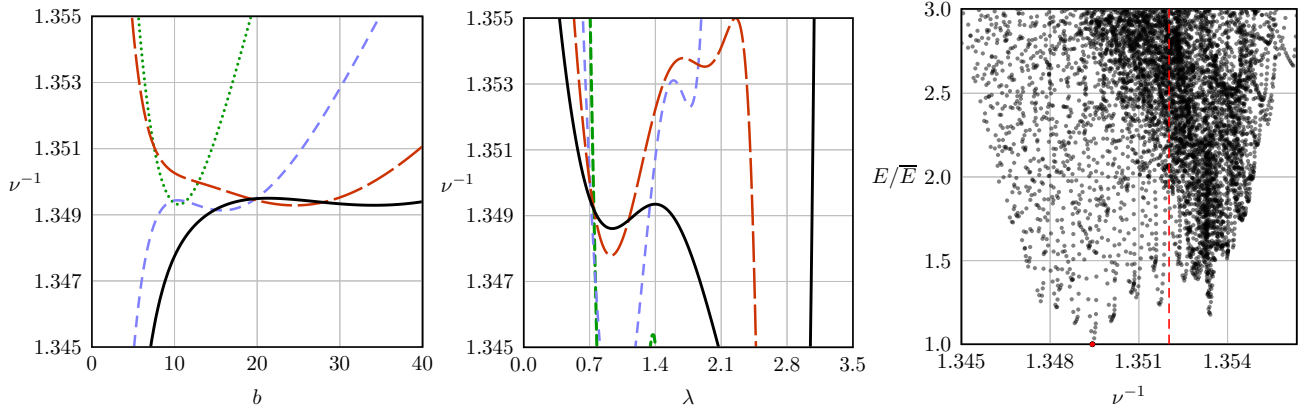

$\omega(n=0)$ : **5 loops**

Minimal error:  $\overline{E} = \overline{E}_5^\omega = 0.00443$  for  $\tilde{\omega}_5^{b,\lambda,q} = 0.83464$  at  $b = 12.5$ ,  $\lambda = 0.54$ ,  $q = 0.52$

$$\delta_5 = 0.00076, \quad \text{Var}_b^{4,5} = 0.00058, \quad \text{Var}_\lambda = 0.00177, \quad \text{Var}_q = 0.00132$$

Weighted mean of  $\tilde{\omega}_5^\theta$  with  $E_5^\omega(\theta) < 3\overline{E}$ : 0.83211, standard deviation:  $\sigma = 0.00313$

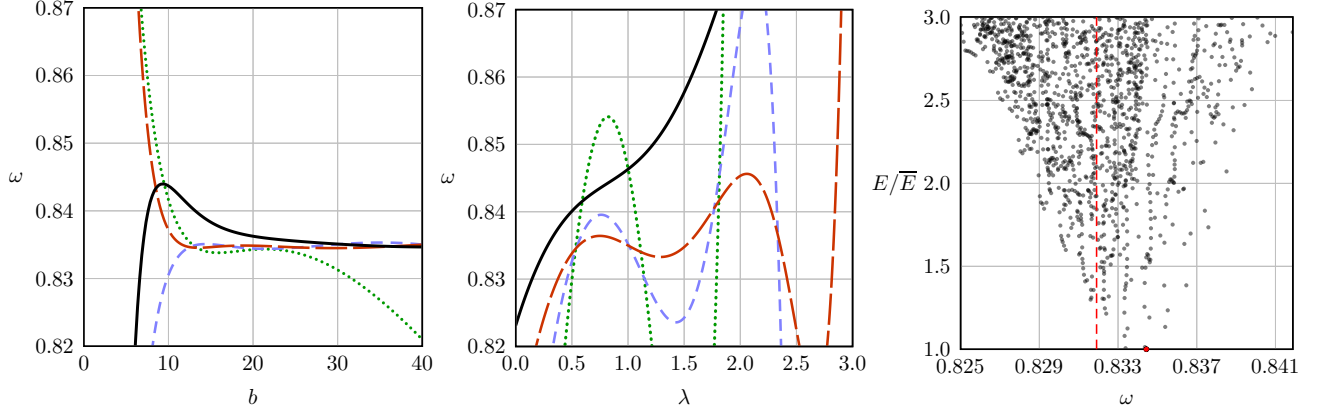

$\omega(n=0)$ : **6 loops**

Minimal error:  $\overline{E} = \overline{E}_6^\omega = 0.00463$  for  $\tilde{\omega}_6^{b,\lambda,q} = 0.84075$  at  $b = 18.0$ ,  $\lambda = 0.48$ ,  $q = 0.60$

$$\delta_6 = 0.00072, \quad \text{Var}_b^{5,6} = 0.00062, \quad \text{Var}_\lambda = 0.00198, \quad \text{Var}_q = 0.00131$$

Weighted mean of  $\tilde{\omega}_6^\theta$  with  $E_6^\omega(\theta) < 3\overline{E}$ : 0.83790, standard deviation:  $\sigma = 0.00420$

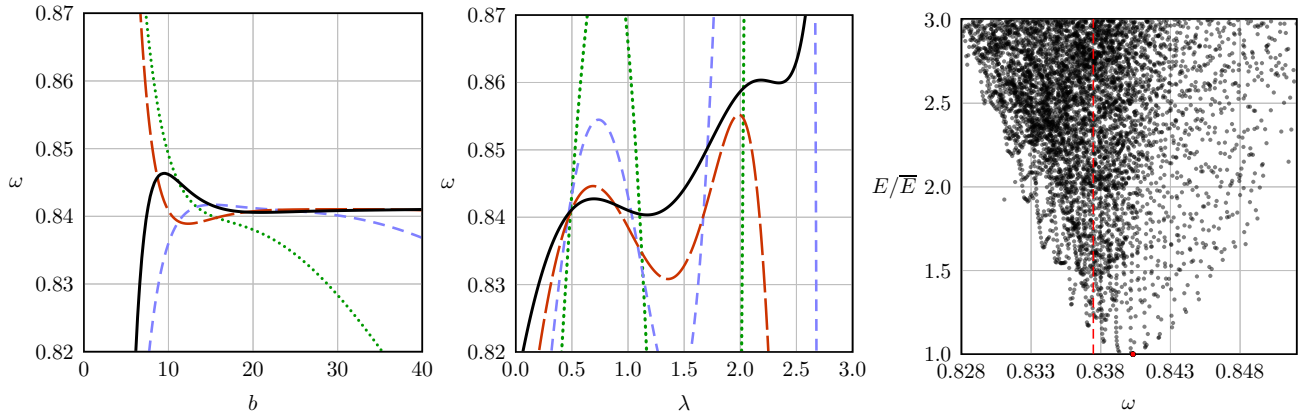

$\omega(n=1)$ : **5 loops**

Minimal error:  $\overline{E} = \overline{E}_5^\omega = 0.00335$  for  $\tilde{\omega}_5^{b,\lambda,q} = 0.81792$  at  $b = 13.0$ ,  $\lambda = 0.58$ ,  $q = 0.40$

$$\delta_5 = 0.00042, \quad \text{Var}_b^{4,5} = 0.00074, \quad \text{Var}_\lambda = 0.00117, \quad \text{Var}_q = 0.00102$$

Weighted mean of  $\tilde{\omega}_5^\theta$  with  $E_5^\omega(\theta) < 3\overline{E}$ : 0.81622, standard deviation:  $\sigma = 0.00216$

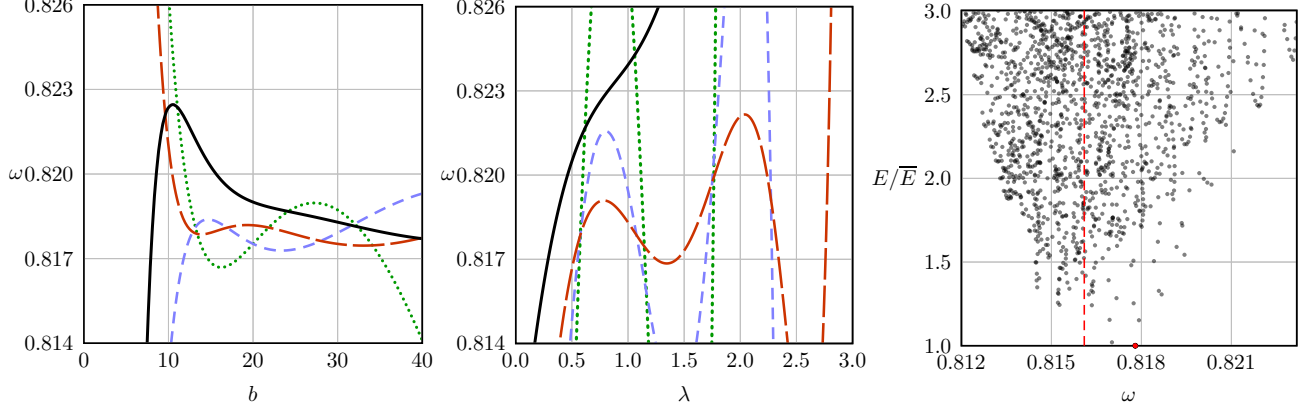

$\omega(n=1)$ : **6 loops**

Minimal error:  $\overline{E} = \overline{E}_6^\omega = 0.00234$  for  $\tilde{\omega}_6^{b,\lambda,q} = 0.81999$  at  $b = 21.5$ ,  $\lambda = 1.02$ ,  $q = 0.40$

$$\delta_6 = 0.00011, \quad \text{Var}_b^{5,6} = 0.00098, \quad \text{Var}_\lambda = 0.00082, \quad \text{Var}_q = 0.00043$$

Weighted mean of  $\tilde{\omega}_6^\theta$  with  $E_6^\omega(\theta) < 3\overline{E}$ : 0.82041, standard deviation:  $\sigma = 0.00219$

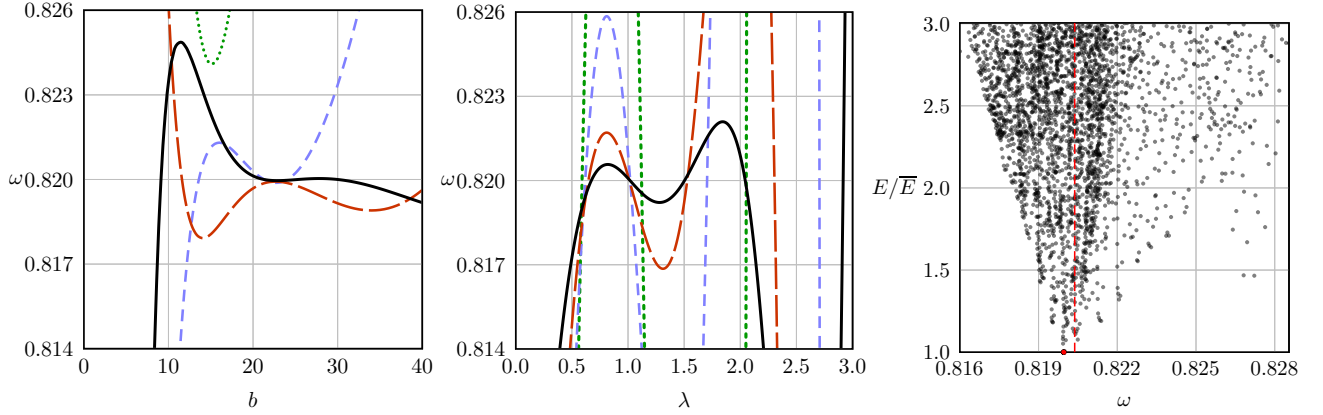

$\omega(n=2)$ : **5 loops**

Minimal error:  $\overline{E} = \overline{E}_5^\omega = 0.00262$  for  $\tilde{\omega}_5^{b,\lambda,q} = 0.80263$  at  $b = 13.5$ ,  $\lambda = 0.80$ ,  $q = 0.18$

$$\delta_5 = 0.00009, \quad \text{Var}_b^{4,5} = 0.00141, \quad \text{Var}_\lambda = 0.00044, \quad \text{Var}_q = 0.00069$$

Weighted mean of  $\tilde{\omega}_5^\theta$  with  $E_5^\omega(\theta) < 3\overline{E}$ : 0.80386, standard deviation:  $\sigma = 0.00175$

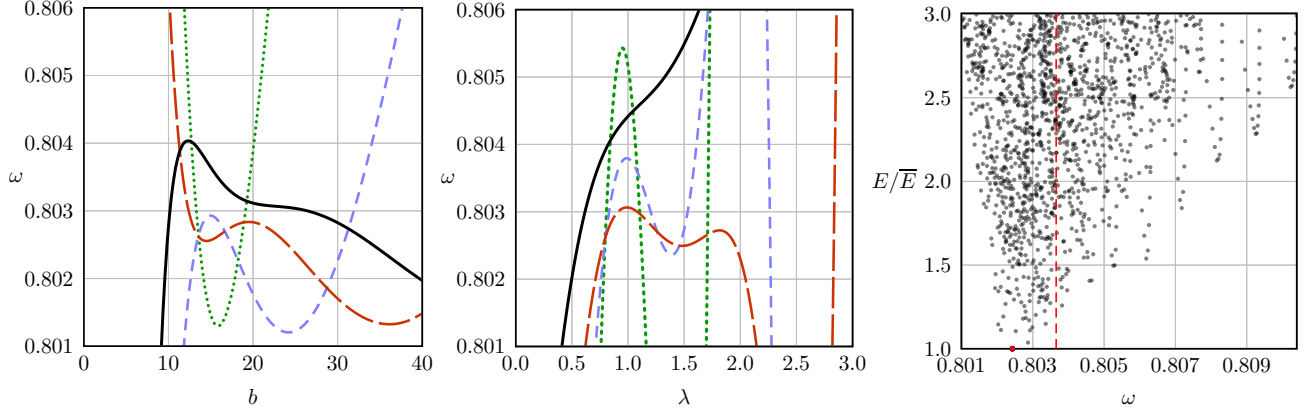

$\omega(n=2)$ : **6 loops**

Minimal error:  $\overline{E} = \overline{E}_6^\omega = 0.00157$  for  $\tilde{\omega}_6^{b,\lambda,q} = 0.80351$  at  $b = 18.5$ ,  $\lambda = 0.90$ ,  $q = 0.18$

$$\delta_6 = 0.00009, \quad \text{Var}_b^{5,6} = 0.00086, \quad \text{Var}_\lambda = 0.00015, \quad \text{Var}_q = 0.00047$$

Weighted mean of  $\tilde{\omega}_6^\theta$  with  $E_6^\omega(\theta) < 3\overline{E}$ : 0.80438, standard deviation:  $\sigma = 0.00083$

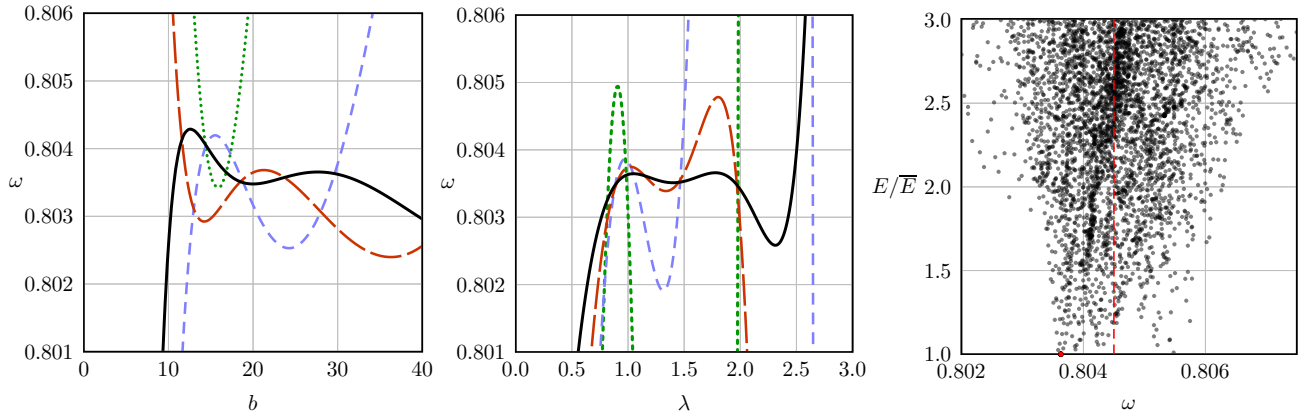

$\omega(n=3)$ : **5 loops**

Minimal error:  $\overline{E} = \overline{E}_5^\omega = 0.00270$  for  $\tilde{\omega}_5^{b,\lambda,q} = 0.79703$  at  $b = 20.0$ ,  $\lambda = 0.84$ ,  $q = 0.10$

$$\delta_5 = 0.00015, \quad \text{Var}_b^{4,5} = 0.00113, \quad \text{Var}_\lambda = 0.00055, \quad \text{Var}_q = 0.00086$$

Weighted mean of  $\tilde{\omega}_5^\theta$  with  $E_5^\omega(\theta) < 3\overline{E}$ : 0.79762, standard deviation:  $\sigma = 0.00206$

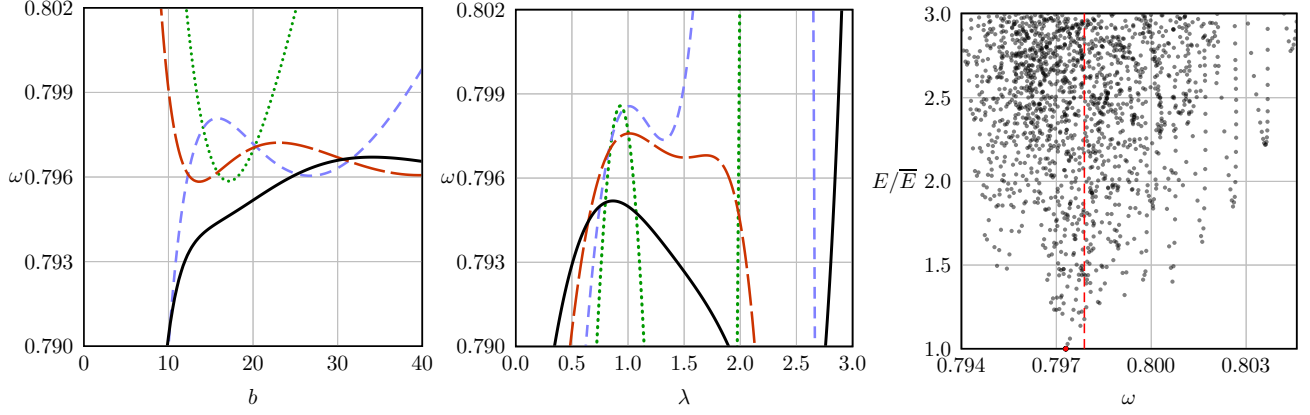

$\omega(n=3)$ : **6 loops**

Minimal error:  $\overline{E} = \overline{E}_6^\omega = 0.00290$  for  $\tilde{\omega}_6^{b,\lambda,q} = 0.79674$  at  $b = 30.5$ ,  $\lambda = 0.86$ ,  $q = 0.10$

$$\delta_6 = 0.00015, \quad \text{Var}_b^{5,6} = 0.00156, \quad \text{Var}_\lambda = 0.00040, \quad \text{Var}_q = 0.00079$$

Weighted mean of  $\tilde{\omega}_6^\theta$  with  $E_6^\omega(\theta) < 3\overline{E}$ : 0.79511, standard deviation:  $\sigma = 0.00199$

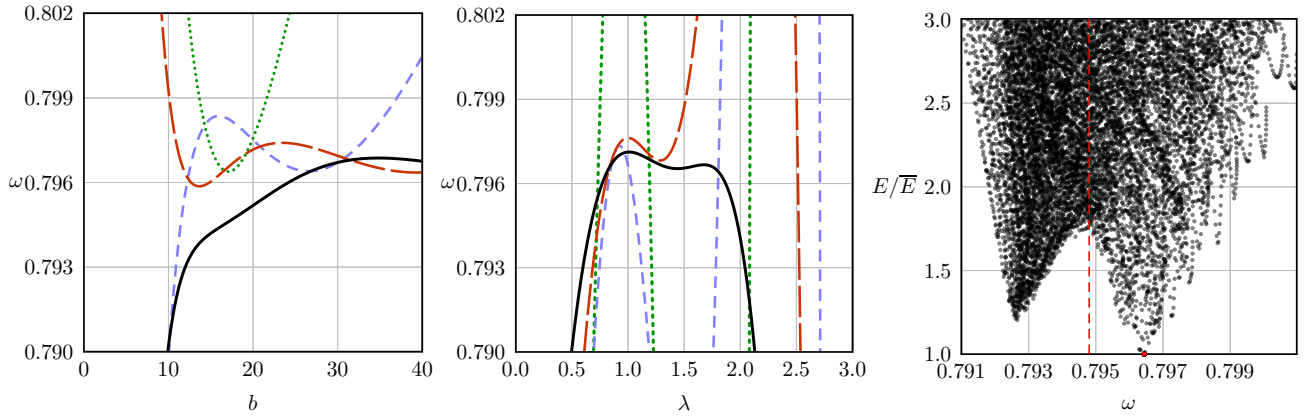

$\omega(n=4)$ : **5 loops**

Minimal error:  $\overline{E} = \overline{E}_5^\omega = 0.00254$  for  $\tilde{\omega}_5^{b,\lambda,q} = 0.79467$  at  $b = 22.5$ ,  $\lambda = 0.94$ ,  $q = 0.02$

$$\delta_5 = 0.00015, \quad \text{Var}_b^{4,5} = 0.00136, \quad \text{Var}_\lambda = 0.00027, \quad \text{Var}_q = 0.00075$$

Weighted mean of  $\tilde{\omega}_5^\theta$  with  $E_5^\omega(\theta) < 3\overline{E}$ : 0.79584, standard deviation:  $\sigma = 0.00177$

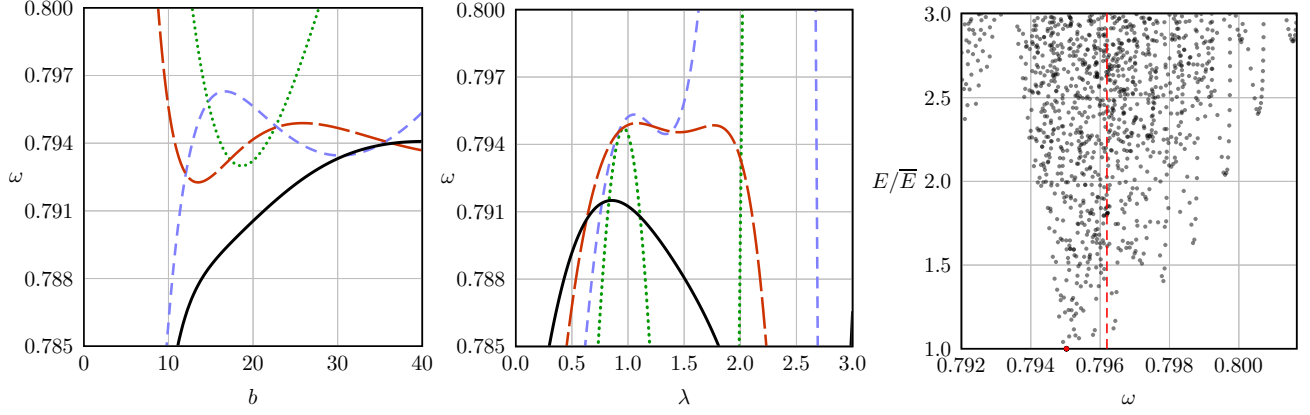

$\omega(n=4)$ : **6 loops**

Minimal error:  $\overline{E} = \overline{E}_6^\omega = 0.00438$  for  $\tilde{\omega}_6^{b,\lambda,q} = 0.79373$  at  $b = 35.0$ ,  $\lambda = 0.90$ ,  $q = 0.02$

$$\delta_6 = 0.00016, \quad \text{Var}_b^{5,6} = 0.00307, \quad \text{Var}_\lambda = 0.00037, \quad \text{Var}_q = 0.00078$$

Weighted mean of  $\tilde{\omega}_6^\theta$  with  $E_6^\omega(\theta) < 3\overline{E}$ : 0.79296, standard deviation:  $\sigma = 0.00240$

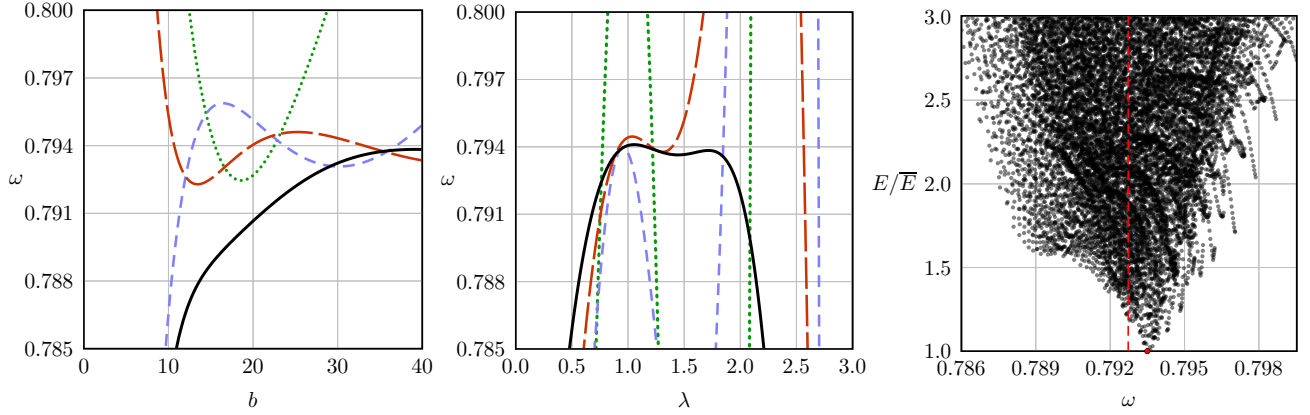



## $D = 2$ dimensions

### $\eta(n = -1)$ : 5 loops

Minimal error:  $\overline{E} = \overline{E}_5^\eta = 0.00711$  for  $\tilde{\eta}_5^{b,\lambda,q} = 0.13713$  at  $b = 7.0$ ,  $\lambda = 2.58$ ,  $q = 0.22$

$$\delta_5 = 0.00003, \quad \text{Var}_b^{4,5} = 0.00306, \quad \text{Var}_\lambda = 0.00083, \quad \text{Var}_q = 0.00320$$

Weighted mean of  $\tilde{\eta}_5^\theta$  with  $E_5^\eta(\theta) < 3\overline{E}$ : 0.13935, standard deviation:  $\sigma = 0.00808$

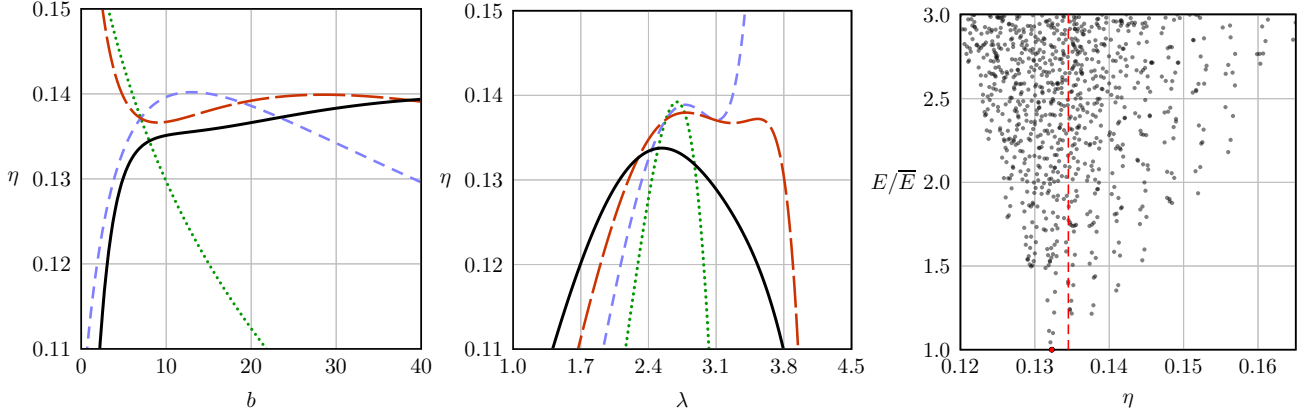

### $\eta(n = -1)$ : 6 loops

Minimal error:  $\overline{E} = \overline{E}_6^\eta = 0.00406$  for  $\tilde{\eta}_6^{b,\lambda,q} = 0.13035$  at  $b = 8.5$ ,  $\lambda = 2.60$ ,  $q = 0.18$

$$\delta_6 = 0.00053, \quad \text{Var}_b^{5,6} = 0.00070, \quad \text{Var}_\lambda = 0.00063, \quad \text{Var}_q = 0.00220$$

Weighted mean of  $\tilde{\eta}_6^\theta$  with  $E_6^\eta(\theta) < 3\overline{E}$ : 0.12583, standard deviation:  $\sigma = 0.00654$

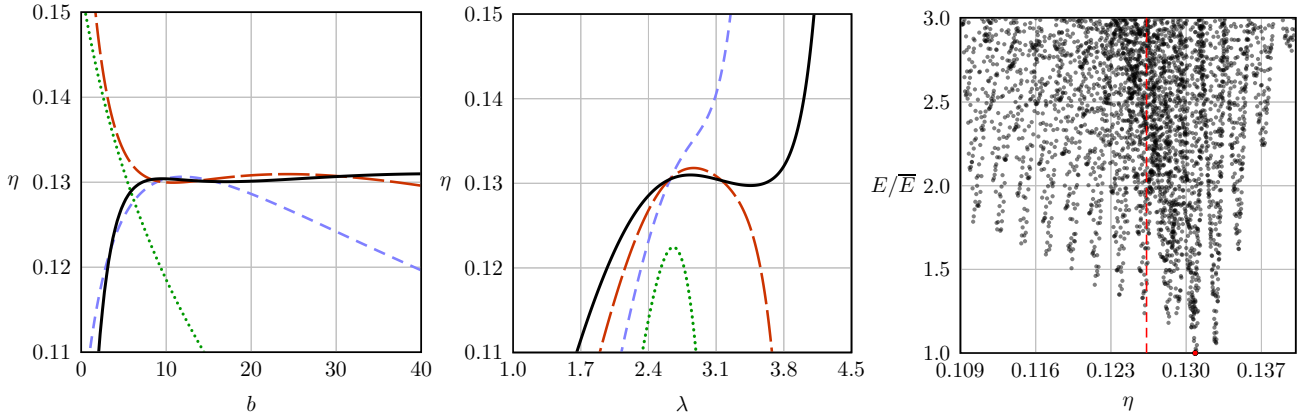

$\eta(n=0)$ : **5 loops**

Minimal error:  $\overline{E} = \overline{E}_5^\eta = 0.01083$  for  $\hat{\eta}_5^{b,\lambda,q} = 0.21472$  at  $b = 7.5$ ,  $\lambda = 2.50$ ,  $q = 0.24$

$$\delta_5 = 0.00083, \quad \text{Var}_b^{4,5} = 0.00309, \quad \text{Var}_\lambda = 0.00172, \quad \text{Var}_q = 0.00519$$

Weighted mean of  $\hat{\eta}_5^\theta$  with  $E_5^\eta(\theta) < 3\overline{E}$ : 0.21599, standard deviation:  $\sigma = 0.01192$

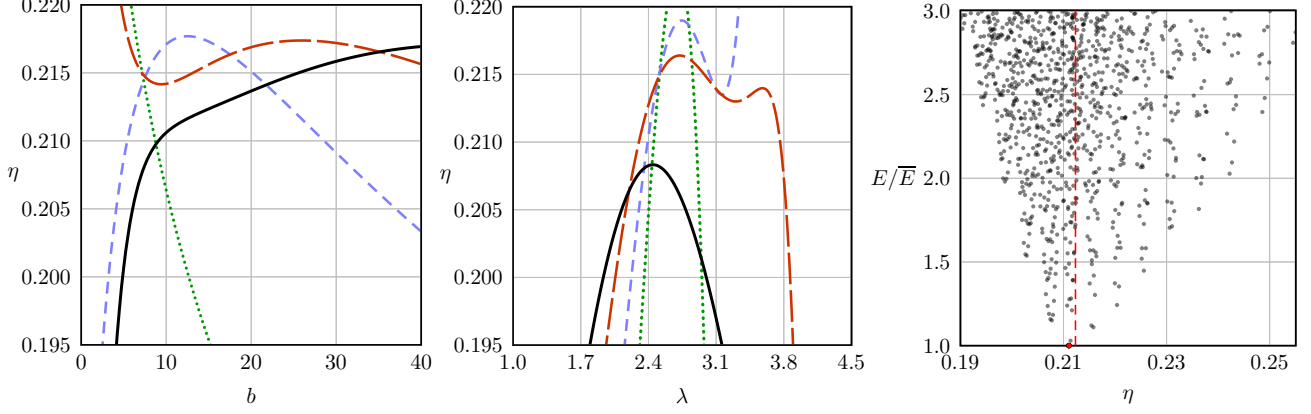

$\eta(n=0)$ : **6 loops**

Minimal error:  $\overline{E} = \overline{E}_6^\eta = 0.00587$  for  $\hat{\eta}_6^{b,\lambda,q} = 0.20093$  at  $b = 10.0$ ,  $\lambda = 2.64$ ,  $q = 0.18$

$$\delta_6 = 0.00013, \quad \text{Var}_b^{5,6} = 0.00161, \quad \text{Var}_\lambda = 0.00086, \quad \text{Var}_q = 0.00328$$

Weighted mean of  $\hat{\eta}_6^\theta$  with  $E_6^\eta(\theta) < 3\overline{E}$ : 0.19447, standard deviation:  $\sigma = 0.00946$

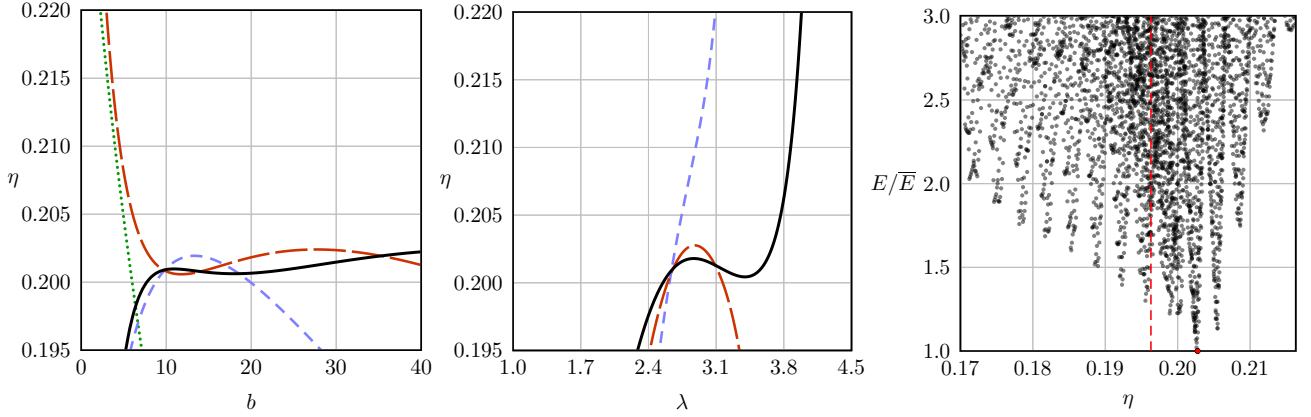

$\eta(n=1)$ : **5 loops**

Minimal error:  $\overline{E} = \overline{E}_5^\eta = 0.01180$  for  $\hat{\eta}_5^{b,\lambda,q} = 0.24889$  at  $b = 8.0$ ,  $\lambda = 2.50$ ,  $q = 0.24$

$$\delta_5 = 0.00053, \quad \text{Var}_b^{4,5} = 0.00366, \quad \text{Var}_\lambda = 0.00188, \quad \text{Var}_q = 0.00573$$

Weighted mean of  $\hat{\eta}_5^\theta$  with  $E_5^\eta(\theta) < 3\overline{E}$ : 0.25112, standard deviation:  $\sigma = 0.01308$

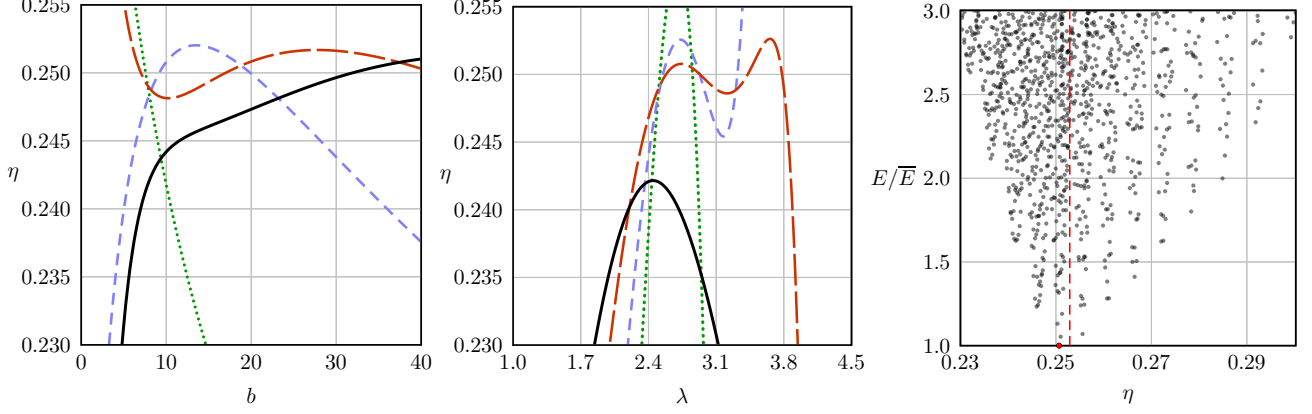

$\eta(n=1)$ : **6 loops**

Minimal error:  $\overline{E} = \overline{E}_6^\eta = 0.00636$  for  $\hat{\eta}_6^{b,\lambda,q} = 0.23709$  at  $b = 11.5$ ,  $\lambda = 2.56$ ,  $q = 0.20$

$$\delta_6 = 0.00015, \quad \text{Var}_b^{5,6} = 0.00104, \quad \text{Var}_\lambda = 0.00109, \quad \text{Var}_q = 0.00407$$

Weighted mean of  $\hat{\eta}_6^\theta$  with  $E_6^\eta(\theta) < 3\overline{E}$ : 0.22859, standard deviation:  $\sigma = 0.01054$

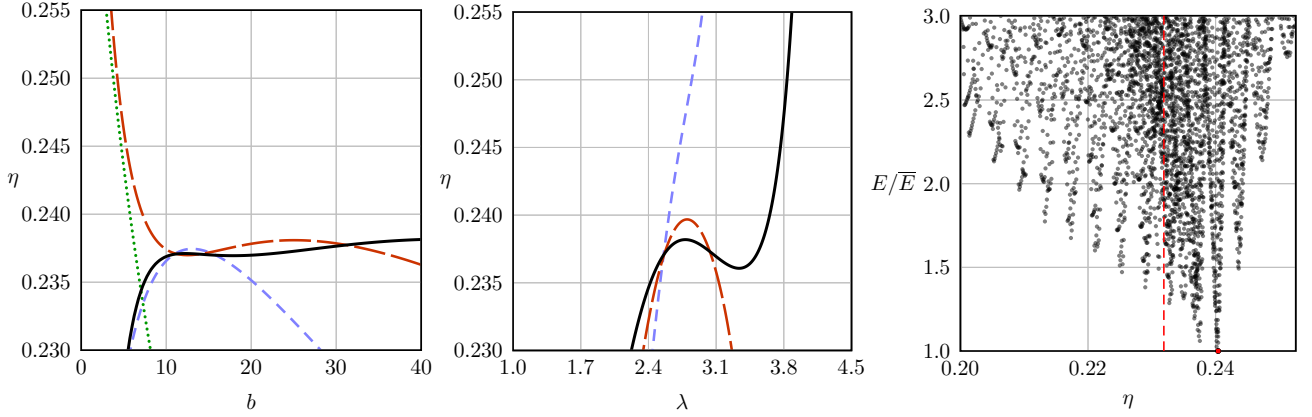

$\nu^{-1}(n = -1)$ : **5 loops**

Minimal error:  $\overline{E} = \overline{E}_5^{\nu^{-1}} = 0.00359$  for  $\widetilde{\nu^{-1}}_5^{b,\lambda,q} = 1.65979$  at  $b = 7.5$ ,  $\lambda = 0.94$ ,  $q = 0.00$

$$\delta_5 = 0.00053, \quad \text{Var}_b^{4,5} = 0.00049, \quad \text{Var}_\lambda = 0.00078, \quad \text{Var}_q = 0.00180$$

Weighted mean of  $\widetilde{\nu^{-1}}_5^\theta$  with  $E_5^{\nu^{-1}}(\theta) < 3\overline{E}$ : 1.65855, standard deviation:  $\sigma = 0.00187$

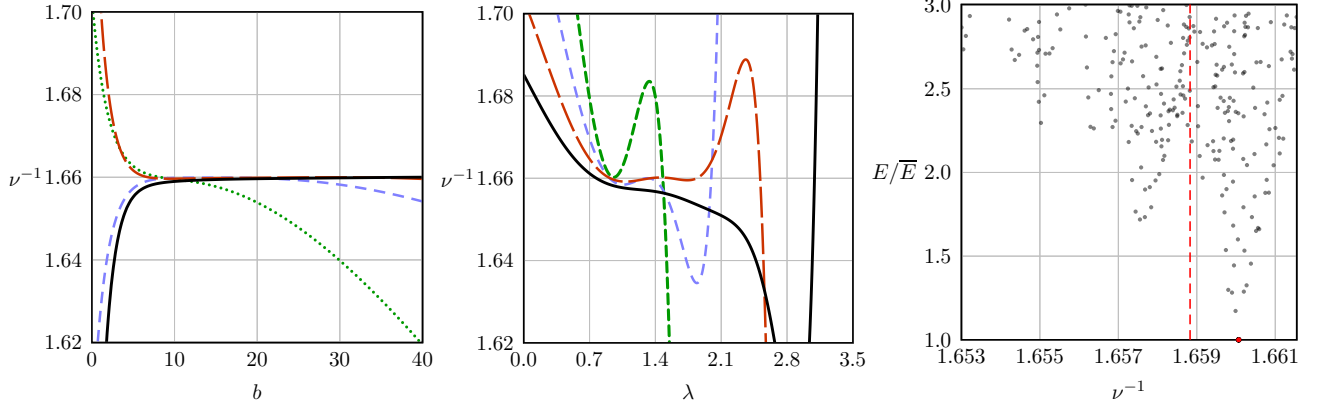

$\nu^{-1}(n = -1)$ : **6 loops**

Minimal error:  $\overline{E} = \overline{E}_6^{\nu^{-1}} = 0.00304$  for  $\widetilde{\nu^{-1}}_6^{b,\lambda,q} = 1.65586$  at  $b = 8.0$ ,  $\lambda = 0.78$ ,  $q = 0.06$

$$\delta_6 = 0.00025, \quad \text{Var}_b^{5,6} = 0.00031, \quad \text{Var}_\lambda = 0.00107, \quad \text{Var}_q = 0.00142$$

Weighted mean of  $\widetilde{\nu^{-1}}_6^\theta$  with  $E_6^{\nu^{-1}}(\theta) < 3\overline{E}$ : 1.65679, standard deviation:  $\sigma = 0.00158$

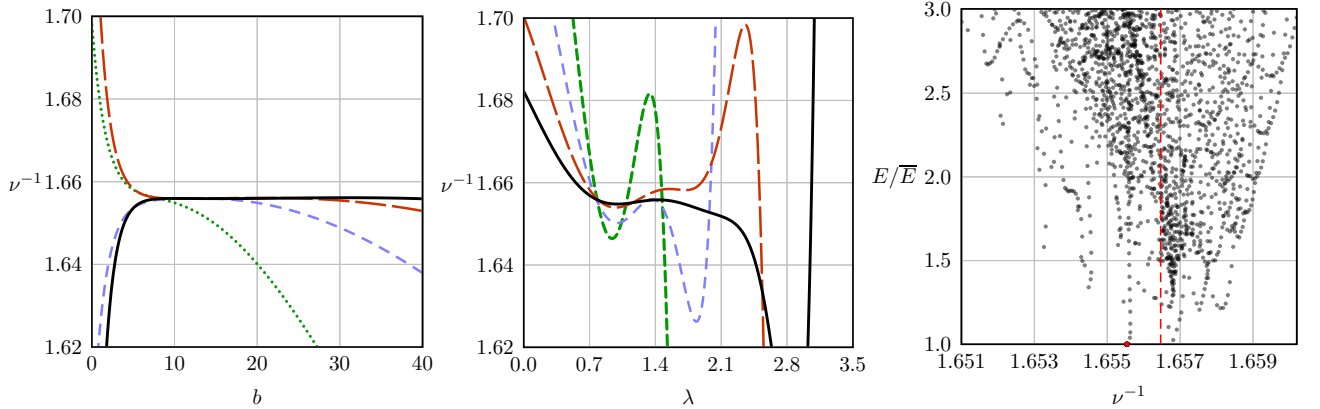

$\nu^{-1}(n=0)$ : **5 loops**

Minimal error:  $\overline{E} = \overline{E}_5^{\nu^{-1}} = 0.01258$  for  $\widetilde{\nu^{-1}}_5^{b,\lambda,q} = 1.35463$  at  $b = 9.0$ ,  $\lambda = 1.48$ ,  $q = 0.00$

$$\delta_5 = 0.00292, \quad \text{Var}_b^{4,5} = 0.00227, \quad \text{Var}_\lambda = 0.00539, \quad \text{Var}_q = 0.00201$$

Weighted mean of  $\widetilde{\nu^{-1}}_5^\theta$  with  $E_5^{\nu^{-1}}(\theta) < 3\overline{E}$ : 1.33804, standard deviation:  $\sigma = 0.01132$

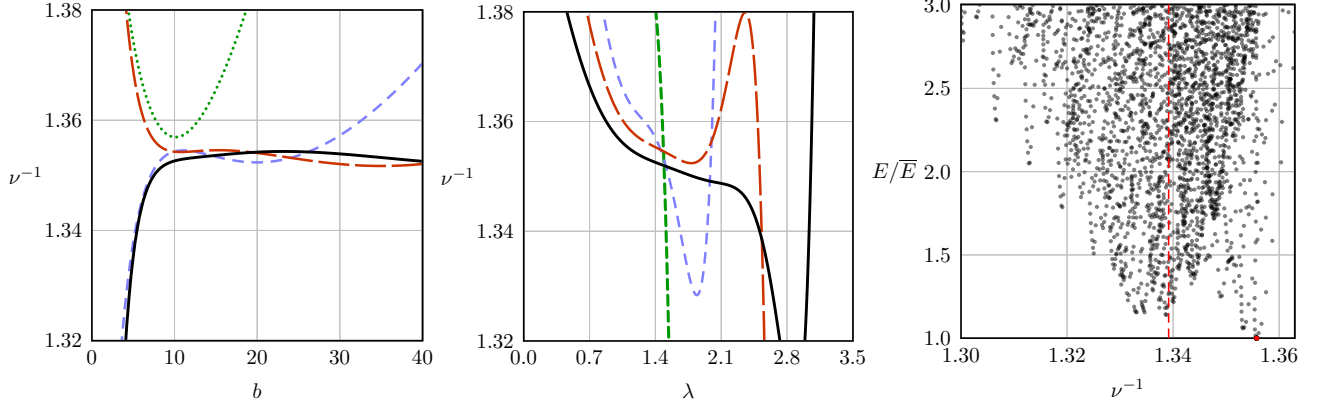

$\nu^{-1}(n=0)$ : **6 loops**

Minimal error:  $\overline{E} = \overline{E}_6^{\nu^{-1}} = 0.00352$  for  $\widetilde{\nu^{-1}}_6^{b,\lambda,q} = 1.34987$  at  $b = 9.5$ ,  $\lambda = 1.42$ ,  $q = 0.04$

$$\delta_6 = 0.00059, \quad \text{Var}_b^{5,6} = 0.00101, \quad \text{Var}_\lambda = 0.00070, \quad \text{Var}_q = 0.00122$$

Weighted mean of  $\widetilde{\nu^{-1}}_6^\theta$  with  $E_6^{\nu^{-1}}(\theta) < 3\overline{E}$ : 1.34913, standard deviation:  $\sigma = 0.00201$

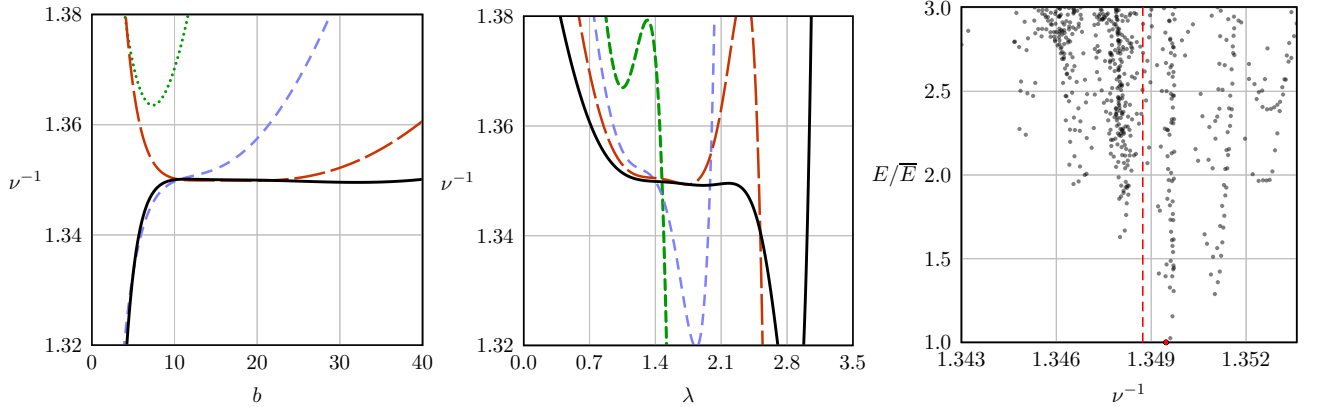

$\nu^{-1}(n=1)$ : **5 loops**

Minimal error:  $\overline{E} = \overline{E}_5^{\nu^{-1}} = 0.01670$  for  $\widetilde{\nu^{-1}}_5^{b,\lambda,q} = 1.05972$  at  $b = 10.0$ ,  $\lambda = 1.46$ ,  $q = 0.12$

$$\delta_5 = 0.00372, \quad \text{Var}_b^{4,5} = 0.00419, \quad \text{Var}_\lambda = 0.00564, \quad \text{Var}_q = 0.00315$$

Weighted mean of  $\widetilde{\nu^{-1}}_5^\theta$  with  $E_5^{\nu^{-1}}(\theta) < 3\overline{E}$ : 1.04783, standard deviation:  $\sigma = 0.01814$

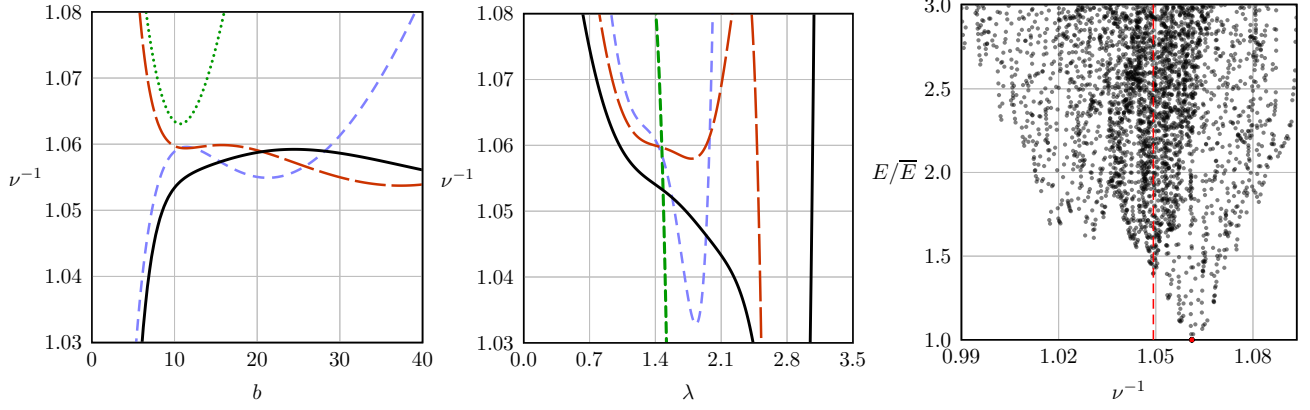

$\nu^{-1}(n=1)$ : **6 loops**

Minimal error:  $\overline{E} = \overline{E}_6^{\nu^{-1}} = 0.00656$  for  $\widetilde{\nu^{-1}}_6^{b,\lambda,q} = 1.05067$  at  $b = 13.0$ ,  $\lambda = 1.32$ ,  $q = 0.16$

$$\delta_6 = 0.00097, \quad \text{Var}_b^{5,6} = 0.00191, \quad \text{Var}_\lambda = 0.00073, \quad \text{Var}_q = 0.00294$$

Weighted mean of  $\widetilde{\nu^{-1}}_6^\theta$  with  $E_6^{\nu^{-1}}(\theta) < 3\overline{E}$ : 1.05136, standard deviation:  $\sigma = 0.00426$

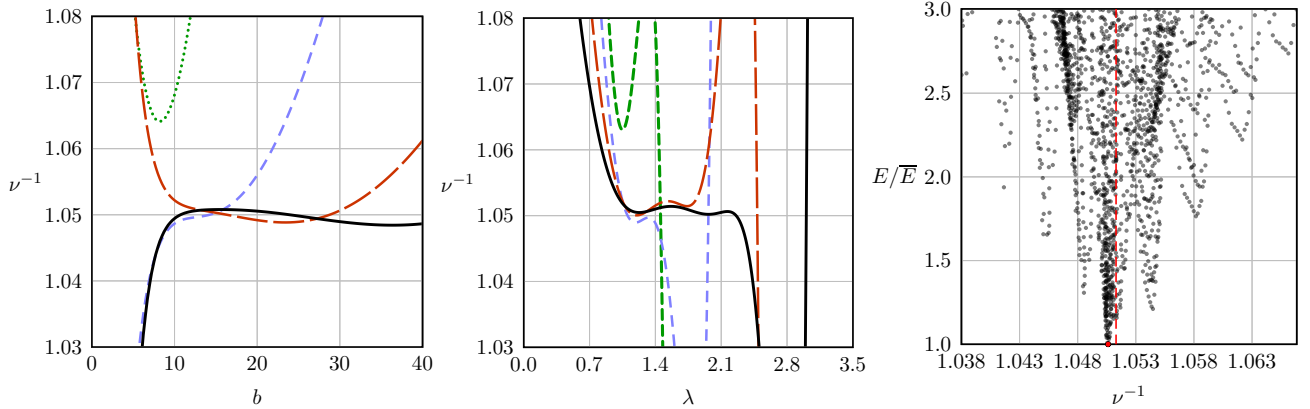

$\omega(n = -1)$ : **5 loops**

Minimal error:  $\overline{E} = \overline{E}_5^\omega = 0.06036$  for  $\tilde{\omega}_5^{b,\lambda,q} = 1.87910$  at  $b = 11.5$ ,  $\lambda = 0.58$ ,  $q = 0.50$

$$\delta_5 = 0.00302, \quad \text{Var}_b^{4,5} = 0.00644, \quad \text{Var}_\lambda = 0.02869, \quad \text{Var}_q = 0.02220$$

Weighted mean of  $\tilde{\omega}_5^\theta$  with  $E_5^\omega(\theta) < 3\overline{E}$ : 1.74658, standard deviation:  $\sigma = 0.12037$

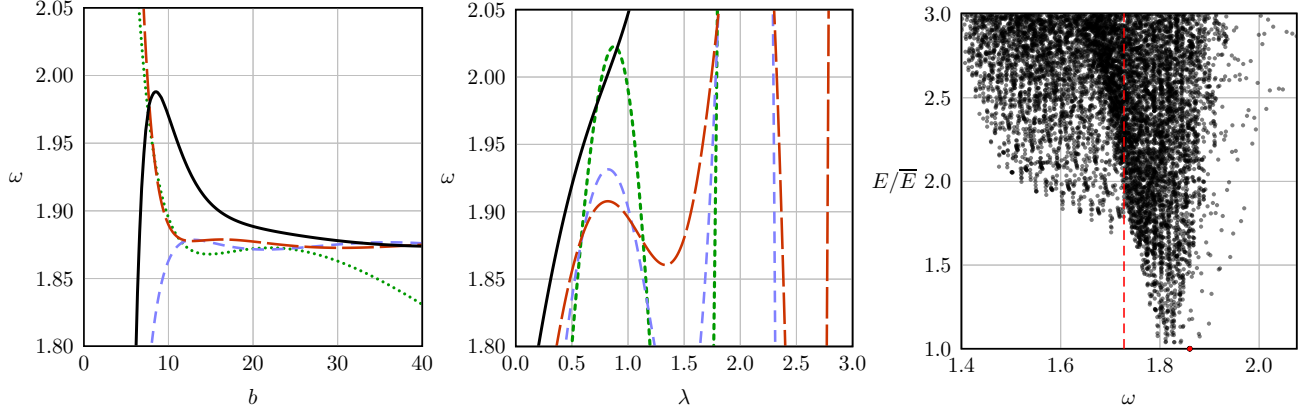

$\omega(n = -1)$ : **6 loops**

Minimal error:  $\overline{E} = \overline{E}_6^\omega = 0.07250$  for  $\tilde{\omega}_6^{b,\lambda,q} = 1.94949$  at  $b = 20.0$ ,  $\lambda = 1.04$ ,  $q = 0.54$

$$\delta_6 = 0.01077, \quad \text{Var}_b^{5,6} = 0.01721, \quad \text{Var}_\lambda = 0.03126, \quad \text{Var}_q = 0.01326$$

Weighted mean of  $\tilde{\omega}_6^\theta$  with  $E_6^\omega(\theta) < 3\overline{E}$ : 1.84276, standard deviation:  $\sigma = 0.10428$

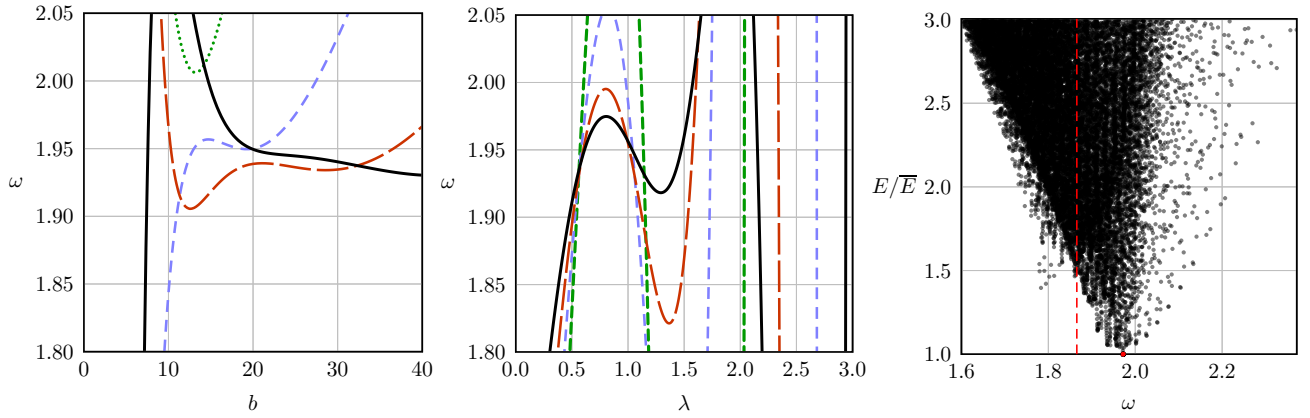

$\omega(n=0)$ : **5 loops**

Minimal error:  $\overline{E} = \overline{E}_5^\omega = 0.05399$  for  $\tilde{\omega}_5^{b,\lambda,q} = 1.83331$  at  $b = 13.0$ ,  $\lambda = 0.56$ ,  $q = 0.50$

$$\delta_5 = 0.00040, \quad \text{Var}_b^{4,5} = 0.00545, \quad \text{Var}_\lambda = 0.02758, \quad \text{Var}_q = 0.02056$$

Weighted mean of  $\tilde{\omega}_5^\theta$  with  $E_5^\omega(\theta) < 3\overline{E}$ : 1.73007, standard deviation:  $\sigma = 0.09736$

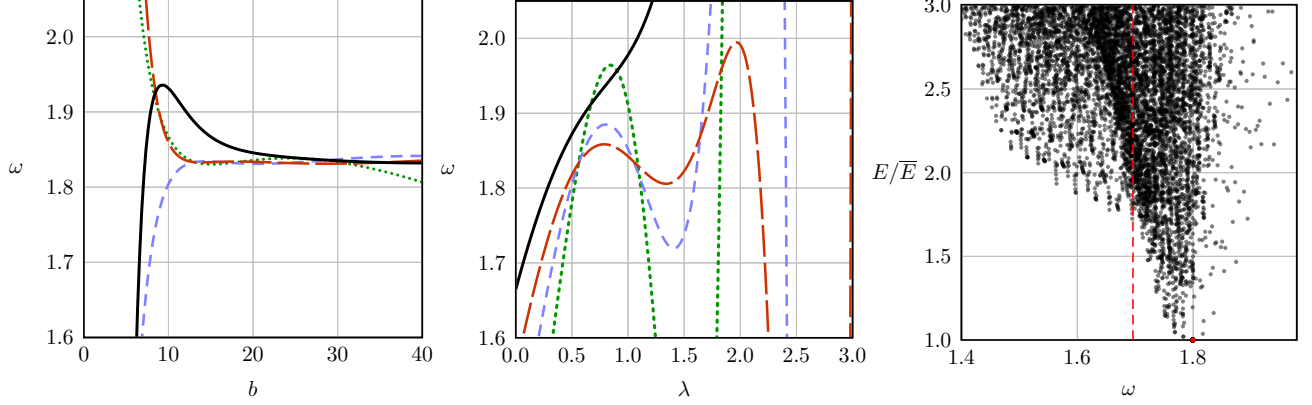

$\omega(n=0)$ : **6 loops**

Minimal error:  $\overline{E} = \overline{E}_6^\omega = 0.06789$  for  $\tilde{\omega}_6^{b,\lambda,q} = 1.90491$  at  $b = 20.0$ ,  $\lambda = 0.52$ ,  $q = 0.56$

$$\delta_6 = 0.00286, \quad \text{Var}_b^{5,6} = 0.00607, \quad \text{Var}_\lambda = 0.03416, \quad \text{Var}_q = 0.02480$$

Weighted mean of  $\tilde{\omega}_6^\theta$  with  $E_6^\omega(\theta) < 3\overline{E}$ : 1.80778, standard deviation:  $\sigma = 0.09236$

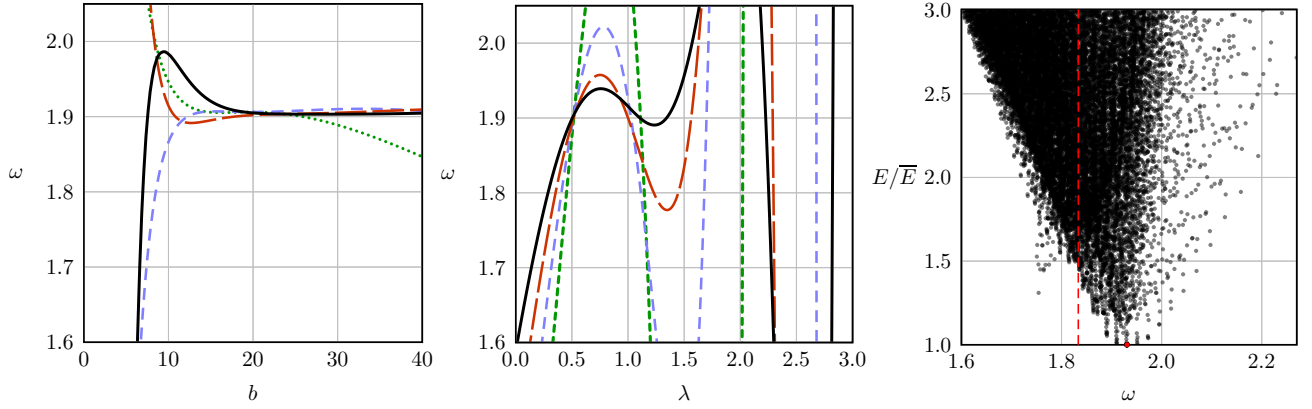



$\omega(n=1)$ : **5 loops**

Minimal error:  $\overline{E} = \overline{E}_5^\omega = 0.03420$  for  $\tilde{\omega}_5^{b,\lambda,q} = 1.67950$  at  $b = 13.0$ ,  $\lambda = 0.60$ ,  $q = 0.38$

$$\delta_5 = 0.00182, \quad \text{Var}_b^{4,5} = 0.00502, \quad \text{Var}_\lambda = 0.01433, \quad \text{Var}_q = 0.01304$$

Weighted mean of  $\tilde{\omega}_5^\theta$  with  $E_5^\omega(\theta) < 3\overline{E}$ : 1.65576, standard deviation:  $\sigma = 0.03562$

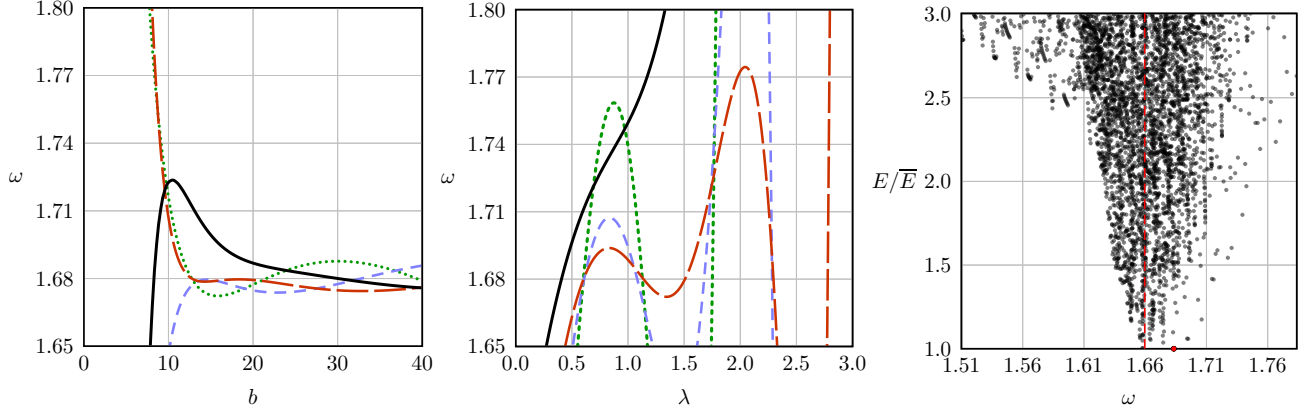

$\omega(n=1)$ : **6 loops**

Minimal error:  $\overline{E} = \overline{E}_6^\omega = 0.02854$  for  $\tilde{\omega}_6^{b,\lambda,q} = 1.70995$  at  $b = 22.0$ ,  $\lambda = 1.02$ ,  $q = 0.40$

$$\delta_6 = 0.00051, \quad \text{Var}_b^{5,6} = 0.00735, \quad \text{Var}_\lambda = 0.01311, \quad \text{Var}_q = 0.00757$$

Weighted mean of  $\tilde{\omega}_6^\theta$  with  $E_6^\omega(\theta) < 3\overline{E}$ : 1.70402, standard deviation:  $\sigma = 0.03256$

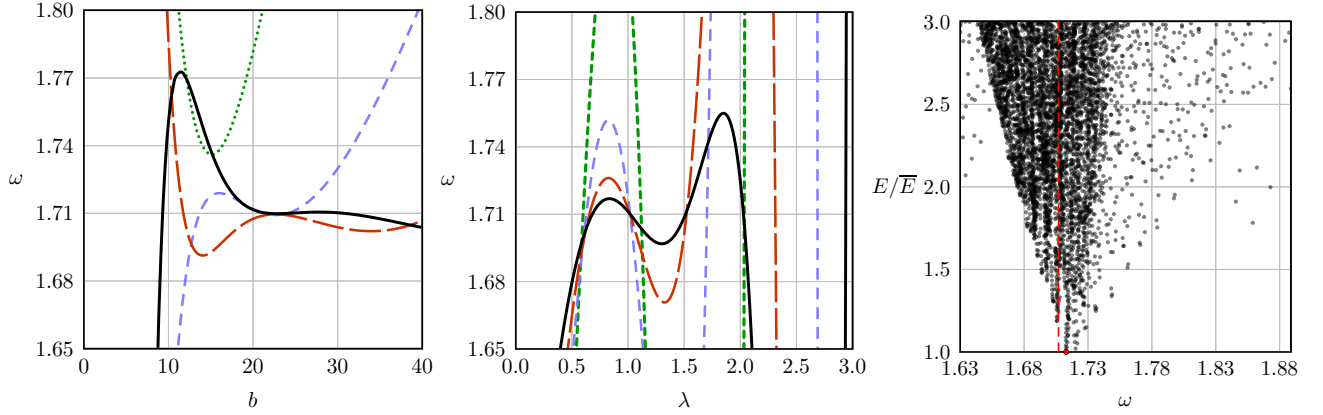

Supplement: Supplementary file 1 [file resummation.pdf]
